# Supplementary material for: Sharp adaptive and pathwise stable similarity testing for scalar ergodic diffusions
Source: arXiv:2203.13776 source file (2024-04-16)
Supplement: Supplementary file 1 [file Appendix_composite.tex]

\section{Appendix D: Composite hypothesis}

\begin{proof}[Proof of Proposition \ref{worst_case_one-sided}]
Let $b\in\mathcal{H}_{\leq}$. The key idea is to split the set $\mathcal{T}$ in three parts: We choose $\delta,\epsilon>0$ and set
\begin{align*}
\mathcal{T}_1 &:= \left\{ (y,h)\in\mathcal{T} \mid h\geq\delta\textrm{ and } \min_{x\in [y-h,y+h]} \rho_b(x)b(x) < - \epsilon\right\}, \\
\mathcal{T}_2 &:_= \left\{ (y,h)\in\mathcal{T} \mid h <\delta\right\}, \textrm{ and }\\
\mathcal{T}_3 &:= \left\{ (y,h)\in\mathcal{T} \mid h\geq\delta\textrm{ and } \rho_b(x)b(x)\geq -\epsilon\textrm{ on } [y-h, y+h]\right\}.
\end{align*}
Note that all sets depend on $\delta$ and $\epsilon$. Then we have
\begin{align*}
\Pr(T_b(X)>r) &= \Pr\left( \sup_{(y,h)\in\mathcal{T}}  \left(  \tilde{\Psi}_{y,h}^b(X) - C(\sigma_{y,h}^2) \right)>r \right) \\
&\leq \Pr\left( \sup_{(y,h)\in\mathcal{T}_1}  \left(  \tilde{\Psi}_{y,h}^b(X) - C(\sigma_{y,h}^2) \right)>r \right)\\
&\hspace{1cm}+\Pr\left( \sup_{(y,h)\in\mathcal{T}_2}  \left(  \tilde{\Psi}_{y,h}^b(X) - C(\sigma_{y,h}^2) \right)>r \right)\\
&\hspace{1cm}+\Pr\left( \sup_{(y,h)\in\mathcal{T}_3}  \left(  \tilde{\Psi}_{y,h}^b(X) - C(\sigma_{y,h}^2) \right)>r \right).
\end{align*}
Of course the inequality remains valid if we put $\lim_{\epsilon\searrow 0}\lim_{\delta\searrow 0}\lim_{T\to\infty}$ before both sides. The rationale behind the argument will be that the first probability converges to zero as the bias in $\tilde{\Psi}$ dominates the stochastic term, the second one vanishes by the multiscale lemma as in the proof of the weak convergence in Theorem \ref{weak_conv} and the last one smaller in stochastic order than $S$. Furthermore, we have seen in Theorem \ref{weak_conv} that both randoms variables $T_b(X)$ and $S$ are $\geq 0$ almost surely and it suffices to consider $r>0$(\textbf{for the first two sumands in $S$ this follows from Theorem \ref{weak_conv}, the third one is positive and bounded by a constant}).

\begin{itemize}
\item[(1)] We can bound $T_b(X)$ with the supremum taken over $\mathcal{T}_1$ by
\[ \sup_{(y,h)\in\mathcal{T}_1} \left( \frac{\frac{1}{\sqrt{T}} \int_0^T K_{y,h}(X_s) dW_s}{\sqrt{\frac1T \int_0^T K_{y,h}(X_s)^2 ds}}  - C(\sigma_{y,h}^2)\right) + \sup_{(y,h)\in\mathcal{T}_1}\frac{\frac{1}{\sqrt{T}} \int_0^T K_{y,h}(X_s)b(X_s) ds}{\sqrt{\frac1T \int_0^T K_{y,h}(X_s)^2 ds}}.\]
The limit in distribution of the first term is given in Theorem \ref{weak_conv} and we are going to show that the second term converges to $-\infty$ almost surely. Then we can conclude
\[ \lim_{T\to\infty} \Pr\left( \sup_{(y,h)\in\mathcal{T}_1}  \left(  \tilde{\Psi}_{y,h}^b(X) - C(\sigma_{y,h}^2) \right)>r \right) =0.\]
First of all we write with the occupation times formula
\[ \frac{\frac{1}{\sqrt{T}} \int_0^T K_{y,h}(X_s)b(X_s) ds}{\sqrt{\frac1T \int_0^T K_{y,h}(X_s)^2 ds}} = \sqrt{T}\frac{\int_\R K_{y,h}(z) b(z) \frac1T L_T^z dz}{\sqrt{\int_\R K_{y,h}(z)^2 \frac1T L_T^z dz}}.\]
We have almost sure convergence of the fraction against
\[ \frac{\int_\R K_{y,h}(z) b(z)\rho_b(z) dz}{\sqrt{\int_\R K_{y,h}(z)^2 \rho_b(z) dz}} = \sqrt{h} \frac{\int_\R K(z) b(y+hz) \rho_b(y+hz)dz}{\sqrt{\int_\R K(z)^2 \rho_b(y+hz)dz}}\]
where equality follows from substitution. Keeping in mind that the expression is negative, upper-bounding it is the same as finding lower bounds of the absolute value. In particular, we may choose the denominator as large as possible by using the upper bound $L^*$ of the invariant density from Lemma \ref{bound_invariant_density} and choosing $h$ as small as possible. Thus we find
\[  \frac{\int_\R K_{y,h}(z) b(z)\rho_b(z) dz}{\sqrt{\int_\R K_{y,h}(z)^2 \rho_b(z) dz}}\leq \sqrt{\delta} \left( \sqrt{L^*} \|K\|_{L^2}\right)^{-1} \int_\R K(z) b(y+hz) \rho_b(y+hz)dz.\]
From our condition on the set $\mathcal{T}_1$ we can find $z' \in [-1,1]$ such that $b(y+hz')\rho_b(y+hz')\leq -\epsilon$. As $b\rho_b$ is a continuous function on $[-A,A]$, it is uniformly continuous. Hence we find $\delta'>0$ (not depending on $y$ and $h$ which is the important part!) such that $b(y+hz)\rho_b(y+hz) <\frac{\epsilon}{2}$ for all $z$ that suffice $|y+hz' - y+hz| <\delta'$. This latter condition is equivalent to $|z-z'|\leq \frac{\delta'}{h}$. We get
\begin{align*}
\int_\R K(z) b(y+hz) \rho_b(y+hz)dz &\leq  - \frac{\epsilon}{2}\int_{B_{\frac{\delta'}{h}}(z')\cap [-1,1]} K(z) dz\\
&\leq  - \frac{\epsilon}{2}\int_{B_{\frac{\delta'}{\delta}}(z')\cap [-1,1]} K(z) dz.
\end{align*}
As $K$ is given by the triangular kernel that integral is minimized for $B_{\frac{\delta'}{\delta}}(z')\cap [-1,1] = [-1, -1+\frac{\delta'}{\delta}]$. As a triangle with both sides $\frac{\delta'}{\delta}$ its volume equals $\frac12 \left(\frac{\delta'}{\delta}\right)^2$ which finally gives
\[ \frac{\int_\R K_{y,h}(z) b(z)\rho_b(z) dz}{\sqrt{\int_\R K_{y,h}(z)^2 \rho_b(z) dz}}\leq -\sqrt{\delta} \left( \sqrt{L^*} \|K\|_{L^2}\right)^{-1}\frac{\epsilon}{4} \left(\frac{\delta'}{\delta}\right)^2\]
and consequently
\[\sqrt{T}\frac{\int_\R K_{y,h}(z) b(z) \frac1T L_T^z dz}{\sqrt{\int_\R K_{y,h}(z)^2 \frac1T L_T^z dz}} \rightarrow_{as} -\infty.\]
As the bound derived for the second factor does not depend on the location parameters $(y,h)$ we can put the supremum before the expression and are done with the first case.

\item[(2)] As the second summand in $\tilde{\Psi}$ is negative, we may disregard it whereby we make the probability of overshooting greater and get from Theorem \ref{weak_conv} that
\begin{align*}
&\lim_{T\to\infty} \Pr\left( \sup_{(y,h)\in\mathcal{T}_2}  \left(  \tilde{\Psi}_{y,h}^b(X) - C(\sigma_{y,h}^2) \right)>r \right) \\
&\hspace{0.5cm}\leq \lim_{T\to\infty} \Pr\left( \sup_{(y,h)\in\mathcal{T}_2}  \left(  \tilde{\Psi}_{y,h}^0(X) - C(\sigma_{y,h}^2) \right)>r \right) \\
&\hspace{0.5cm} = \Pr\left( \sup_{(y,h)\in\mathcal{T}_2} \left( \frac{\int_{-A}^A K_{y,h}(z) \sqrt{\rho_b(z)} dW_z}{\| K_{y,h}\sqrt{\rho_b}\|_{L^2}} - C(\left( \|K_{y,h}\sqrt{\rho_b}\|_{L^2}^2\right)\right) >r\right)
\end{align*}
Now $\|K_{y,h}\|_{L^2}^2 = h\|K\|_{L^2}^2$ and we have in the notation of Theorem \ref{weak_conv}
\[ \lim_{\delta\searrow 0}\lim_{T\to\infty} \Pr\left( \sup_{(y,h)\in\mathcal{T}_2}  \left(  \tilde{\Psi}_{y,h}^b(X) - C(\sigma_{y,h}^2) \right)>r \right) \leq \lim_{\delta\searrow 0}\lim_{T\to\infty}\Pr\left( S(0,\delta)>r\right) =0.\]

\item[(3)] For the last part we first drop the condition $h\geq \delta$ and get
\[ \mathcal{T}_3\subset \left\{ (y,h)\in\mathcal{T}\mid \rho_b(x)b(x)\geq -\epsilon\textrm{ on } [y-h,y+h]\right\} =: \mathcal{T}_3'\]
which particularly implies
\begin{align*}
\Pr\left( \sup_{(y,h)\in\mathcal{T}_3}  \left(  \tilde{\Psi}_{y,h}^b(X) - C(\sigma_{y,h}^2) \right)>r \right)&\leq \Pr\left( \sup_{(y,h)\in\mathcal{T}_3'}  \left(  \tilde{\Psi}_{y,h}^b(X) - C(\sigma_{y,h}^2) \right)>r \right)\\
&\leq \Pr\left( \sup_{(y,h)\in\mathcal{T}_3'}  \left(  \tilde{\Psi}_{y,h}^0(X) - C(\sigma_{y,h}^2) \right)>r \right),
\end{align*} 
where we again dropped the second summand of $\tilde{\Psi}$ in the second step as it is negative for $b\in\mathcal{H}_{\leq}$. By the weak limit in Theorem \ref{weak_conv}
\begin{align*}
&\lim_{T\to\infty} \Pr\left( \sup_{(y,h)\in\mathcal{T}_3}  \left(  \tilde{\Psi}_{y,h}^b(X) - C(\sigma_{y,h}^2) \right)>r \right)\\
&\hspace{1cm} = \Pr\left( \sup_{(y,h)\in\mathcal{T}_3'} \left(\frac{\int_{-A}^A K_{y,h}(z)\sqrt{\rho_b(z)} dW_z}{\| K_{y,h}\sqrt{\rho_b}\|_{L^2}} - C\left( \|K_{y,h}\sqrt{\rho_b}\|_{L^2}^2\right)\right) >r\right).
\end{align*}
Taking the limit $\lim_{\delta\searrow 0}$ doesn't change anything as neither side depends on $\delta$ and it remains to evaluate $\lim_{\epsilon\searrow 0}$.
If we write $\mathcal{T}_3'(\epsilon)=\mathcal{T}_3'$ we see that $\mathcal{T}_3'(\epsilon)\subset \mathcal{T}_3'(\epsilon')$ for $\epsilon\leq \epsilon'$ and 
\[ \lim_{\epsilon\searrow 0} \mathcal{T}_3'(\epsilon) = \left\{ (y,h)\in\mathcal{T}\mid \rho_b b=0 \textrm{ on } [y-h, y+h]\right\} =:\mathcal{T}_3''.\]
For each $(y,h)\in\mathcal{T}_3''$ we have that $\rho_b=c$ is constant on $[y-h,y+h]$ as $\rho_b'=\frac{2b\rho_b}{\sigma^2}$ and thus
\begin{align*}
&\lim_{\epsilon\searrow 0} \sup_{(y,h)\in\mathcal{T}_3'(\epsilon)} \left(\frac{\int_{-A}^A K_{y,h}(z)\sqrt{\rho_b(z)} dW_z}{\| K_{y,h}\sqrt{\rho_b}\|_{L^2}} - C\left( \|K_{y,h}\sqrt{\rho_b}\|_{L^2}^2\right)\right)\\
&\hspace{1cm} = \sup_{(y,h)\in\mathcal{T}_3''} \left(\frac{\int_{-A}^A K_{y,h}(z)dW_z}{\| K_{y,h}\|_{L^2}} - C\left( \|K_{y,h}c\|_{L^2}^2\right)\right)\\
&\hspace{1cm} \leq  \sup_{(y,h)\in\mathcal{T}_3''} \left(\frac{\int_{-A}^A K_{y,h}(z)dW_z}{\| K_{y,h}\|_{L^2}} - C\left( \|\tilde{c}K_{y,h}\|_{L^2}^2\right)\right)
\end{align*} 
with $\tilde{c} = 1\vee (L^*\wedge \frac{1}{2h})$. Here we used in the last step that $c\leq L^*$ is clear, as the invariant density is bounded by $L^*$. Furthermore, as it integrates to one, we have $2hc\leq 1\Leftrightarrow c\leq \frac{1}{2h}$. Finally, the reasoning is finished by noting that $C(\cdot)$ decreases with increasing argument. \\
For any $a>b>0$ we have $\sqrt{a-b}\geq \sqrt{a}-\sqrt{b}$ as
\[ (\sqrt{a}-\sqrt{b})^2 = a - 2\sqrt{ab}+b \leq a-2b+b = a-b.\]
By the definition of $C(\cdot)$ and the calculus rules of $\log$ we thus have
\begin{align*}
C\left( \|\tilde{c}K_{y,h}\|_{L^2}^2\right) &= \sqrt{2\log\left(\frac{1}{\tilde{c}K_{y,h}\|_{L^2}^2}\right)}\\
&= \sqrt{ 2\log\left( \frac{1}{\|K_{y,h}\|_{L^2}^2}\right) - 2\log(\tilde{c})} \\
&\geq  \sqrt{ 2\log\left( \frac{1}{\|K_{y,h}\|_{L^2}^2}\right)}  - \sqrt{2\log(\tilde{c})}\\
&= C(\|K_{y,h}\|_{L^2}^2) - C(\tilde{c}^{-1})
\end{align*}
Furthermore, we increase the random variable, by taking the supremum over a larger set, in this case $\mathcal{T}$ instead of $\mathcal{T}_3''$. This gives
\[\lim_{\epsilon\searrow 0} \sup_{(y,h)\in\mathcal{T}_3'(\epsilon)} \left(\frac{\int_{-A}^A K_{y,h}(z)\sqrt{\rho_b(z)} dW_z}{\| K_{y,h}\sqrt{\rho_b}\|_{L^2}} - C\left( \|K_{y,h}\sqrt{\rho_b}\|_{L^2}^2\right)\right) \leq S.\]
Altogether, we have
\[ \lim_{\epsilon\searrow 0}\lim_{\delta\searrow 0}\lim_{T\to\infty}\Pr\left( \sup_{(y,h)\in\mathcal{T}_3}  \left(  \tilde{\Psi}_{y,h}^b(X) - C(\sigma_{y,h}^2) \right)>r \right) \leq \Pr\left( S>r\right).\]
\end{itemize}
\end{proof}

\begin{proof}[Proof of Theorem \ref{theorem_one-sided}]
For part (a) define the hypotheses as in the proof of Theorem \ref{lower_bound} with $b_0= 0$ within the interval $[-A,A]$ and $\beta=1$. Then follow the lines of the proof.\\
For part (b) note that the probability of rejecting the null hypothesis is bounded from below by $\Pr_b\left( T_b(X) >\kappa_{\leq,\alpha}\right)\geq \Pr_b\left( \tilde{\Psi}_{y,h}^b(X) > \kappa_{\leq,\alpha} + C(\sigma_{y,h}^2) \right)$ which equals
\begin{align*}
\Pr\left( \frac{\frac{1}{\sqrt{T}} \int_0^T K_{y,h}(X_s) dW_s}{\sqrt{\frac1T \int_0^T K_{y,h}(X_s)^2 ds}} >  +\kappa_{\leq,\alpha} + C(\sigma_{y,h}^2)-\frac{\frac{1}{\sqrt{T}} \int_0^T K_{y,h}(X_s)b(X_s) ds}{\sqrt{\frac1T \int_0^T K_{y,h}(X_s)^2 ds}}\right)
\end{align*}
As in the proof of Theorem \ref{Upper_bound} the left-hand side is tight and the left-hand side goes to $-\infty$ which follows the same lines and makes use of the fact that for $\beta=1$ the rectangular kernel is exactly the optimal recovery kernel used in Theorem \ref{Upper_bound}. The claim follows.
\end{proof}

\begin{proof}[Proof of Proposition \ref{worst_case_delta}]
The idea of the proof is the same as in the proof of Proposition \ref{worst_case_one-sided}. We choose $\epsilon, \epsilon'>0$ and set
\begin{align*}
\mathcal{T}_1 &:= \left\{ (y,h)\in\mathcal{T} \mid h\geq\epsilon'\textrm{ and } \min_{x\in [y-h,y+h]} \rho_b(x)(|b(x)-b_0(x)|-\delta) < - \epsilon\right\}, \\
\mathcal{T}_2 &:_= \left\{ (y,h)\in\mathcal{T} \mid h <\epsilon'\right\}, \textrm{ and }\\ 
\mathcal{T}_3 &:= \left\{ (y,h)\in\mathcal{T} \mid h\geq\epsilon'\textrm{ and } \rho_b(x)(|b(x)-b_0(x)|-\delta)\geq -\epsilon\textrm{ on } [y-h, y+h]\right\}.
\end{align*}
As in the proof of Proposition \ref{worst_case_one-sided} upper-bound the probability $\Pr_b(T_\delta(X)>r)$ by the sum of the overshooting probabilities for each $\sup_{\mathcal{T}_i}$ and then take $\lim_{\epsilon\searrow 0}\lim_{\epsilon'\searrow 0}\lim_{T\to\infty}$ on both sides.
Before we start with the three summands, we note that $|\Psi_{y,h}(X)| - \Psi_\delta $ is upper bounded by
\[ \left|\frac{\frac{1}{\sqrt{T}} \int_0^T K_{y,h}(X_s) dW_s}{\sqrt{\frac1T \int_0^T K_{y,h}(X_s)^2 ds}} \right|+ \frac{\left|\frac{1}{\sqrt{T}}\int_0^T K_{y,h}(X_s) ( b(X_s) - b_0(X_s)) ds\right|-\frac{\delta}{\sqrt{T}} \int_0^T K_{y,h}(X_s) ds}{\sqrt{\frac1T \int_0^T K_{y,h}(X_s)^2 ds}}. \]
Using the triangle inequality, the numerator of the second summand is smaller than
\[ \frac{1}{\sqrt{T}} \int_0^T K_{y,h}(X_s) \left( |b(X_s) -b_0(X_s)| -\delta\right) ds\]
and this term is small than zero for each $b\in\mathcal{H}_\delta(b_0)$ and hence the whole second summand. 
\begin{enumerate}
\item[(1)] We bound $T_\delta(X)$ with the supremum taken over $\mathcal{T}_1$ by
\begin{align*}
&\sup_{(y,h)\in\mathcal{T}_1}\left( \left|\frac{\frac{1}{\sqrt{T}} \int_0^T K_{y,h}(X_s) dW_s}{\sqrt{\frac1T \int_0^T K_{y,h}(X_s)^2 ds}} \right| - C(\sigma_{y,h})\right)\\
&\hspace{1cm} + \sup_{(y,h)\in\mathcal{T}_1} \frac{ \frac{1}{\sqrt{T}} \int_0^T K_{y,h}(X_s) \left( |b(X_s) -b_0(X_s)| -\delta\right) ds}{\sqrt{\frac1T \int_0^T K_{y,h}(X_s)^2 ds}}.
\end{align*} 
The distribution of the first term is given in Theorem \ref{weak_conv} and we show convergence of the second term to $-\infty$. Now we repeat the arguments of part (1) in the proof of \ref{worst_case_one-sided}: Applying the occupation times formula, using almost sure convergence and bounding the nominator. Then the second summand without the supremum is given by $\sqrt{T}$ times an expression that is negative and can be upper-bounded by
\[ \sqrt{\epsilon'}\left(\sqrt{L*}\|K\|_{L^2}\right)^{-1} \int_\R K(z)\left( |b(y+hz)-b_0(y+hz)|-\delta\right)\rho_b(y+hz) dz.\]
Now $\left( |b(y+hz)-b_0(y+hz)|-\delta\right)\rho_b(y+hz)$ is $\leq-\epsilon$ at some point and we apply the same uniform continuity argument as in \ref{worst_case_one-sided} to find the uniform in $(y,h)$ upper bound
\[ -\sqrt{\epsilon'}\left(\sqrt{L*}\|K\|_{L^2}\right)^{-1}\frac{\epsilon}{4}\left( \frac{\eta}{\epsilon'}\right)^2,\]
for suitable $\eta>0$ (that plays the role of $\delta'$ in the other proof).

\item[(2)] By neglecting the second negative summand in $T_\delta(X)$ we may estimate
\begin{align*}
&\Pr\left( \sup_{(y,h)\in\mathcal{T}_2} \left( \Psi_{y,h}(X) - C(\sigma_{y,h}^2) - \Psi_\delta\right) >r\right)\\
&\hspace{1cm}\leq \Pr\left( \sup_{(y,h)\in\mathcal{T}_2} \left( \left|\frac{\frac{1}{\sqrt{T}} \int_0^T K_{y,h}(X_s) dW_s}{\sqrt{\frac1T \int_0^T K_{y,h}(X_s)^2 ds}} \right| - C(\sigma_{y,h}^2)\right)>r\right).
\end{align*}
By the same argument as in part (2) of the proof of \ref{worst_case_one-sided} using Theorem \ref{Multiscale_Lemma} we then get
\[ \lim_{\epsilon'\searrow 0}\lim_{T\to\infty} \Pr\left( \sup_{(y,h)\in\mathcal{T}_2} \left( \Psi_{y,h}(X) - C(\sigma_{y,h}^2) - \Psi_\delta\right) >r\right) =0.\]

\item[(3)] Here we again drop the negative summand and for the remaining term get the weak limit
\[ \sup_{(y,h)\in\mathcal{T}_3} \left(\left|\frac{\int_{-A}^A K_{y,h}(z)\sqrt{\rho_b(z)} dW_z}{\| K_{y,h}\sqrt{\rho_b}\|_{L^2}}\right| - C\left( \|K_{y,h}\sqrt{\rho_b}\|_{L^2}^2\right)\right).\]
Now we make the term larger by forgetting about the condition on $\epsilon'$ in $\mathcal{T}_3$, and thus $\lim_{\epsilon'\searrow 0}$ does not change anything. Then we may take the limit $\lim_{\epsilon\searrow 0}$ and are left with those $(y,h)$ for which $b$ behaves either as $b_0 + \delta$ or $b_0-\delta$ on $[y-h,y+h]$, one case corresponding to $S_1$, the other to $S_2$, respectively. Thus, the maximum $S_1\vee S_2$ dominates the term stochastically and we are done.
\end{enumerate}
\end{proof}

\begin{proof}[Proof of Theorem \ref{theorem_delta}]
For part (a) define the hypotheses as in the proof of Theorem \ref{lower_bound} with $b_0$ replaced by $b_0+\delta\in\Sigma(C,A,\gamma,\sigma)$ and $\beta=1$. Then follow the lines of the proof.\\
For part (b) note that the probability of rejecting the null hypothesis is bounded from below by 
\[\Pr_b\left( T_\delta(X) >\kappa_{\leq,\alpha}\right)\geq \Pr_b\left( |\Psi_{y,h}(X)| > \kappa_{\leq,\alpha} + C(\sigma_{y,h}^2)+\Psi_\delta \right)\]
which in turn is bounded by
\begin{align*}
&\Pr\left( \left|\frac{\frac{1}{\sqrt{T}} \int_0^T K_{y,h}(X_s) dW_s}{\sqrt{\frac1T \int_0^T K_{y,h}(X_s)^2 ds}}\right| <-\kappa_{\leq,\alpha} - C(\sigma_{y,h}^2)\right.\\
&\hspace{1cm} \left.  + \frac{\frac{1}{\sqrt{T}} \left|\int_0^T K_{y,h}(X_s)\left(b(X_s)-b_0(X_s)\right) ds\right| -\frac{\delta}{\sqrt{T}}\int_0^T K_{y,h}(X_s) ds}{\sqrt{\frac1T \int_0^T K_{y,h}(X_s)^2 ds}}  \right)
\end{align*}
As in the proof of Theorem \ref{Upper_bound} the left-hand side is tight and we are done if we can establish that the right hand side tends to $\infty$. Let $y$ be the point, where
\[  (|b(y)-b_0(y)| - \delta) \rho_b(y)^\frac13 > L^\frac13 \rho_T\]
and define 
\[ h_T :=  L^{-\frac23}\left( \frac{\log T}{T\rho_b(y)}\right)^\frac13.\]
For large enough $T$ we know by the Lipschitz condition on $b-b_0$ that it has the same sign on the support of $K_{y,h_T}$. Hence, the right-hand side is given by
\[ \frac{\frac{1}{\sqrt{T}} \int_0^T K_{y,h}(X_s)\left(\left|b(X_s)-b_0(X_s)\right|-\delta\right) ds}{\sqrt{\frac1T \int_0^T K_{y,h}(X_s)^2 ds}}.\]
Now we use the occupation times formular, the Hölder class condition on $|b-b_0|-\delta$ and the fact that for $\beta=1$ the rectangular kernel is the optimal recovery kernel and proceed as in the proof Theorem \ref{Upper_bound}.
\end{proof}
