# Supplementary material for: Sharp adaptive and pathwise stable similarity testing for scalar ergodic diffusions
Source: arXiv:2203.13776 source file (2024-04-16)
Supplement: Supplementary file 2 [file Appendix_Preliminary_lemma.tex]

\section{Preliminaries on scalar ergodic diffusion processes}\label{App_prelim}

This section is organized as follows: In Subsection~\ref{A1_SubSec} we state important preliminary results about ergodic diffusions that are given as solutions to stochastic differential equations of the form \eqref{eq: SDE}. Most of them can be found in the literature, but some of those related to the drift function class $\Sigma(C,A,\gamma,\sigma)$ are our own work. The corresponding proofs can be found in Subsection~\ref{A2_SubSec}. In the third part~\ref{A3_SubSec} we give details on how Proposition \ref{moments_local-invariant}, which is given below and taken from the literature, can be transferred to diffusions not started in the invariant measure, but in a fixed point $X_0=x_0$.

\subsection{Preliminary results on scalar ergodic diffusion processes}\label{A1_SubSec}

Following Section~\ref{Sec_Notation}, we consider the stochastic differential equation~\eqref{eq: SDE} of the form
\[ dX_t = b(X_t) dt + \sigma dW_t, \quad X_0=\xi\]
for a standard Brownian motion $W$, initial condition $\xi\sim\mu_b$ independent of $W$ and a drift function $b$ belonging to the class $\Sigma(C,A,\gamma,\sigma)$. We recall its definition for fixed constants $A,\gamma, \sigma >0$ and $C\geq 1$,
\begin{align*}
\Sigma(C,A,\gamma, \sigma) &:=\left\{ b\in \textrm{Lip}_\textrm{loc}(\R):\ |b(x)|\leq C(1+|x|)\ \forall x\in\R \textcolor{white}{\frac12} \right.\\
&\hspace{3cm}\left.\textrm{ and } \frac{b(x)}{\sigma^2}\textrm{sign}(x)\leq -\gamma\ \forall |x|\geq A\right\}.
\end{align*}
Here, $\textrm{Lip}_\textrm{loc}(\R)$ denotes the class of all functions $f:\R\rightarrow\R$ such that for every $n\in\N$ there exists a constant $L_n>0$ such that 
\[ |f(x) - f(y)| \leq L_n |x-y|\quad \textrm{ for all } x,y\textrm{ with } |x|,|y|\leq n. \]
As noted in Section~\ref{Sec_Notation}, for each $b\in\Sigma(C,A,\gamma,\sigma)$ the diffusion $X$ admits the invariant density
\[ q_b(x) := \frac{1}{C_{b,\sigma} } \exp\left( \int_0^x \frac{2b(u)}{\sigma^2} du\right) \quad\textrm{ for all } x\in\R,\]
with the normalizing constant 
\[ C_{b,\sigma}:= \int_\R \exp\left(\int_0^x \frac{2b(u)}{\sigma^2} du\right)dx,\]
where for $x<0$ the integrals should be read as $\int_0^x f(u)du = -\int_{x}^0 f(u) du$.
Some regularity properties of $q_b$ are already determined by $b$. In particular, it is easily seen that $q_b$ is differentiable and for all $x\in\R$,
\[q_b'(x) = 2\sigma^{-2}b(x) q_b(x).\]
Moreover, an important property that is made use of in several steps, is that $q_b$ and $q_b'$ can be uniformly upper bounded over $\Sigma(C,A,\gamma,\sigma)$, whereas on the other hand on the inverval $[-A,A]$, the invariant density $q_b$ is uniformly bounded away from zero. This is stated in the next two lemmas. Both of them are used in the literature on ergodic diffusions, sometimes with a slight modification of the class of functions under consideration. For completeness and the reader's convenience, a proof taylored to our drift function class $\Sigma(C,A,\gamma,\sigma)$ is given in Subsection~\ref{A2_SubSec} that also delivers explicit constants.

\begin{lemma}\label{bound_invariant_density}
There exists a constant $L^* = L^*(C,A,\gamma,\sigma)<\infty$ such that
\[ \sup_{b\in\Sigma(C,A,\gamma,\sigma)} \max\left\{ \|q_b\|_\infty, \| q_b'\|_\infty\right\} \leq L^*.\]
\end{lemma}

\begin{lemma}\label{uniform_lower_bound_invariant_density}
There exists a constant $L_*=L_*(C,A,\gamma,\sigma)>0$ such that
\[ \inf_{b\in \Sigma(C,A,\gamma,\sigma)} \inf_{x\in [-A,A]} q_b(x)\geq L_*.\]
\end{lemma}

Of particular importance in all statistical applications for ergodic diffusions is the fact that those admit a law of large numbers and a central limit theorem (CLT) as stated below.

\begin{thm}[\cite{Kutoyants}, Theorem $1.16$] \label{ergodic_LLN}
Let $b\in\Sigma(C,A,\gamma,\sigma)$. Then we have for any measurable function $f:\R\rightarrow\R$ with $\E_b[|f(\xi)|]<\infty$ and $T\to\infty$,
\[ \frac1T \int_0^T f(X_t) dt\longrightarrow_{\textrm{as}}\E_b[f(\xi)].\]
\end{thm}

\begin{thm}[\cite{Kutoyants}, Proposition $1.22$] \label{ergodic_CLT}
Let $b\in\Sigma(C,A,\gamma,\sigma)$ and $f$ be a measurable function $f:\R\rightarrow\R$ with $\E_b[f(\xi)^2] <\infty$. Then we have the weak convergence
\[ \frac{1}{\sqrt{T}} \int_0^T f(X_t) dW_t\ \longrightarrow_{\mathcal{D}}\ \mathcal{N}\ \left(0, \int_\R f(z)^2 q_b(z) dz\right).\]
\end{thm}

Another very important concept in the statistical investigation of one-dimensional ergodic diffusion processes is the local time $\left(L_t^z(X)\right)_{t\geq 0}$ of the process $X$. It is uniquely determined by the equation
\[ |X_t - z| = |X_0 - z| + \int_0^t \textrm{sign}(X_s - z) dX_s + L_t^z(X)\]
 (cf. \cite{Durrett}, Section~$2.11$, in particular $(11.1)$ and $(11.2)$). For us, the most important consequence of the concept of local time is that it allows to convert time integrals into integrals with respect to the location parameter via the so called \textit{occupation times formula} stated below for our setting. %Its proof is given in a quite general semimartingal context in the reference.

\begin{thm}[\cite{Durrett}, special case of Theorem $11.7$] \label{occupation_times_formula}
For any bounded measurable function $f:\R\rightarrow\R$ it holds
\[ \int_0^T f(X_t) dt = \sigma^{-2} \int_\R f(z) L_T^z(X) dz.\]
\end{thm} 

%A consequence is the following approximation 
%\[ L_T^z(X) = \lim_{\epsilon\searrow 0} \frac{\sigma^2}{\epsilon}  \int_0^T \1_{[z, z+\epsilon)}(X_t) dt, \]
%which justifies the interpretation of $L_T^z(X)$  as the amount of time spent by $X$ at $z$ until time $T$. This suggests that the averaged local time $\frac{1}{\sigma^2 T} L_T^z(X)$ should be a good approximation of the invariant density $q_b(z)$. Indeed, we have the following result that justifies to call $\frac{1}{\sigma^2 T}L_T^\cdot(X)$ the \textit{empirical density} of $X$.

%\begin{thm}[\cite{vanZanten_2}, Theorem $8$]\label{convergence_empirical_density}
%Let $b\in\Sigma(C,A,\gamma,\sigma)$. Then for every $M>0$ we have
%\[ \sup_{|z|\leq M} \left| \frac{1}{T\sigma^2} L_T^z - q_b(z)\right| \longrightarrow_\textrm{as}\ 0 \quad \textrm{ for }\ T\to\infty.\]
%\end{thm}

%For our applications, the almost sure convergence is not necessary, but we need uniform estimates over the class $\Sigma(C,A,\gamma,\sigma)$. An important result in this context is the following uniform moment bound on the difference of the local time and the invariant density in supremum norm.

Additionally, the normalized local time $\frac{1}{\sigma^2 T} L_T^\cdot (X)$ approximates the invariant density $q_b$ in the following sense.

\begin{proposition}[\cite{Strauch}, Corollary $14$]\label{moments_local-invariant}
Let $b\in\Sigma(C,A,\gamma,\sigma)$. Then there exist constants $c_1, c_2>0$ such that, for any $p, T\geq 1$, 
\begin{align*} 
&\sup_{b\in\Sigma(C,A,\gamma,\sigma)} \left(\E_{b}\left[ \left\| \frac{1}{T\sigma^2} L_T^\cdot(X) - q_b\right\|_\infty^p\right]\right)^\frac1p \\
&\hspace{2.5cm} \leq c_1\left( \frac{p}{T} + \frac{1}{\sqrt{T}}\left( 1+ \sqrt{p} + \sqrt{\log T}\right) + Te^{-c_2T}\right).
\end{align*}
\end{proposition}

\begin{remark}\label{remark_moment_invariant}
The preceeding Proposition~\ref{moments_local-invariant} was proven for our setup where the diffusion $X$ is started in the invariant density. In Section~\ref{Sec_Stability} we need to consider the case where it is started in some fixed $x_0\in\R$ to compare it with a fractional diffusion. For this, it is crucial that our results of Section~\ref{Sec_Power} are still true under this assumption, which is also interesting on its own, see Remark~\ref{remark_fixed_point}. To transfer the results, we show that Proposition~\ref{moments_local-invariant} also works for $X_0=x_0\in [-A,A]$, although some parts of the proof have to be slightly modified. This is explained and given in detail in Subsection~\ref{A3_SubSec}.
\end{remark}

%By Markov's inequality we get as a direct corollary of Proposition~\ref{moments_local-invariant}:

\begin{cor}\label{conv_emprical_density_uniform}
We have uniform stochastic convergence of the empirical density to the true one, i.e. for every $\epsilon>0$,
\[\sup_{b\in\Sigma(C,A,\gamma,\sigma)} \Pr_b\left( \left\| \frac{1}{\sigma^2 T} L_T^z (X) - q_b(z)\right\|_\infty >\epsilon\right) \stackrel{T\to\infty}{\longrightarrow} 0.\]
\end{cor}

With this result, we can deduce a uniform version of the weak law of large numbers for a bounded class of functions having compact support. The proof is also provided in Subsection \ref{A2_SubSec}.

\begin{proposition}\label{uniform_ergodic}
Let $\mathcal{F}$ be a class of functions that are bounded uniformly by some constant $C_\mathcal{F}$ and supported in $[-A,A]$. Then for every $\epsilon>0$,
\[ \lim_{T\to\infty} \sup_{b\in\Sigma(C,A,\gamma,\sigma)} \Pr_b\left( \sup_{f\in\mathcal{F}}\left|\frac1T \int_0^T f(X_s) ds - \int_\R f(z) q_b(z) dz \right| >\epsilon\right) =0.\]
\end{proposition}

The next results provides the Radon-Nikodym derivative of two diffusions satisfying \eqref{eq: SDE} for different drifts taken from $\Sigma(C,A,\gamma,\sigma)$. It is sometimes referred to as a variant of Girsanov's theorem.

\begin{thm}[\cite{Kutoyants}, Theorem $1.12$]\label{Girsanov}
Let $X^1$ denote the solution of \eqref{eq: SDE} with drift $b_1$ up to time $T$ and $X^2$ the corresponding solution of \eqref{eq: SDE} with drift $b_2$, where $b_1,b_2\in\Sigma(C,A,\gamma,\sigma)$. Then their likelihood ratio is given as
\begin{align*}
\frac{d\Pr_{b_2}}{d\Pr_{b_1}}(X) &= \frac{q_{b_2}(X_0)}{q_{b_1}(X_0)} \exp\left( \int_0^T \frac{b_2(X_s) - b_1(X_s)}{\sigma^2} dX_s \right. \\
&\hspace{4cm} \left. - \frac12\int_0^T \frac{b_2(X_s)^2 - b_1(X_s)^2}{\sigma^2} ds \right). 
\end{align*} 
\end{thm}

Last but not least, we state the following result that justifies the choice of the drift function $b_0$ in Theorems \ref{worst_case_delta}, \ref{lower_bound}, \ref{Upper_bound} and \ref{thm_adaptivity}.

\begin{lemma}\label{lemma_b+eta}
Let $\eta>0$ and $b_0\in \Sigma\left(\frac{C}{2}-\eta, A, \gamma+\frac{\eta}{\sigma^2}, \sigma\right)$. Then we have $b_0\pm\eta \in\Sigma\left(\frac{C}{2},A,\gamma,\sigma\right)$.
\end{lemma}

\subsection{Proofs of Subsection~\ref{A1_SubSec}}\label{A2_SubSec}
This subsection comprises the proofs of the results from Subsection \ref{A1_SubSec} that are not taken from the literature.

\begin{proof}[Proof of Lemma \ref{bound_invariant_density}]
Let $b\in\Sigma(C,A,\gamma,\sigma)$. First, we look for an upper bound of the normalizing factor $C_{b,\sigma}^{-1}$ of the invariant density $q_b$, which is equivalent to looking for a lower bound of $C_{b,\sigma}$. By the at most linear growth condition for $b$,
\begin{align}\label{eqp: A4}
\begin{split}
\left| \int_0^x 2\sigma^{-2} b(y) dy\right|& \leq 2\sigma^{-2} \textrm{sign}(x) \int_0^x |b(y)|dy\\
& \leq 2\sigma^{-2} \textrm{sign}(x)\int_0^xC(1+|y|)dy \\
& \leq 2C\sigma^{-2}(1+|x|)|x|.
\end{split}
\end{align} 
As $(1+|x|)|x|$ is increasing in $|x|$, it follows by non-negativity of $\exp(\cdot)$ that
\[ C_{b,\sigma} \geq \int_{-C^{-1}}^{C^{-1}} \exp\left(\int_0^u 2\sigma^{-2} b(y) dy\right) du \geq \frac{2}{C} \exp\left( -2\sigma^{-2}\left(1+C^{-1}\right)\right).\]
Thus,
\begin{align}\label{eqp: A5}
\frac{1}{C_{b,\sigma}} \leq \frac{C}{2} e^{2\sigma^{-2}(1+C^{-1})},
\end{align} 
and the normalizing constant of the invariant density $q_b$ is bounded uniformly over $b\in\Sigma(C,A,\gamma,\sigma)$ by some constant depending only on $C$ and $\sigma$.\\
We now turn to $\exp\left(\int_0^x 2\sigma^{-2} b(y) dy\right)$ and see that it suffices to bound the exponent by some constant. For $x>0$ we use \eqref{eqp: A4} and $\textrm{sign}(x)b(x)\sigma^{-2} \leq -\gamma$ for $|x|>A$, to get
\begin{align*}
\int_0^x 2\sigma^{-2} b(y) dy &= \int_0^{A\wedge x} 2\sigma^{-2}b(y) dy + \int_{A\wedge x}^x 2\sigma^{-2}b(y) dy \\
&\leq 2\sigma^{-2} C(1+A) A + 2\int_{A\wedge x}^x -\gamma dy\\
&= 2\sigma^{-2} C(1+A) A -2\gamma(x-A\wedge x).
\end{align*} 
Similarly, for $x<0$,
\begin{align*}
\int_0^x 2\sigma^{-2} b(y) dy &=  - \int_{x\vee (-A)}^0 2\sigma^{-2}b(y) dy - \int_x^{x\vee (-A)}2\sigma^{-2}b(y) dy\\
%&\leq 2\sigma^{-2} C(1+A)A - 2\int_x^{x\vee (-A)}\gamma dy\\ 
&= 2\sigma^{-2} C(1+A)A - 2\gamma ((x\vee (-A)) - x).
\end{align*}
Putting both estimates together gives
\begin{align}\label{eqp: A1}
\exp\left(\int_0^x 2\sigma^{-2} b(y) dy\right)\leq \exp\left( 2\sigma^{-2}C(1+A)A - 2\gamma\left( |x|-A\right)_+\right),
\end{align}
and finally combined with \eqref{eqp: A5}, we find
\[ q_b(x) \leq \frac{C}{2} e^{2\sigma^{-2}(1+C^{-1})} e^{2\sigma^{-2}C(1+A)A } =: L_1.\]
Next, we turn to $\|q_b'\|_\infty$, where we use $q_b' = 2\sigma^{-2}b q_b$. With the at most linear growth condition on $b$, \eqref{eqp: A5} and \eqref{eqp: A1} we have
\begin{align*}
|q_b'(x)| \leq \left|2\sigma^{-2}b(x) q_b(x)\right| &\leq C\sigma^{-2}e^{2\sigma^{-2}(1+C^{-1})}  C(1+|x|)e^{\tilde{c} - 2\gamma (|x|-A)_+}\\
& \leq C^2\sigma^{-2}e^{2\sigma^{-2}(1+C^{-1})}   \left( e^{\tilde{c}} + |x|e^{\tilde{c} - 2\gamma (|x|-A)_+}\right)
\end{align*} 
with  $\tilde{c} = 2\sigma^{-2}C(1+A)A $. The function $|x| e^{\tilde{c} - 2\gamma(|x|-A)_+}$ is bounded which can be seen as follows: For $|x|\leq A$ we have
\[ |x| e^{\tilde{c} - 2\gamma(|x|-A)_+} = |x| e^{\tilde{c}} \leq Ae^{\tilde{c}}.\]
On the other hand, for $|x|> A$ we have $|x| e^{\tilde{c} - 2\gamma(|x|-A)_+} = |x| e^{\tilde{c} + 2A\gamma - 2\gamma |x|}$.
Basic calculus gives a maximum for $|x|=\frac{1}{2\gamma}$ if $2A\gamma\leq 1$, otherwise the maximum is attained on the boundary $|x|=A$. Consequently,
\[ |q_b'(x)| \leq C^2\sigma^{-2} e^{2\sigma^{-2}(1+C^{-1})}  \left( e^{\tilde{c}} + \left(\frac{1}{2\gamma}e^{\tilde{c}+2A\gamma-1} \vee Ae^{\tilde{c}}\right)\right) =:L_2\]
and the proof is finished by taking $L^* := L_1\vee L_2$.
\end{proof}

\begin{proof}[Proof of Lemma \ref{uniform_lower_bound_invariant_density}]
In \eqref{eqp: A4} we have seen that for $x\in [-A,A]$,
\[ \left| \int_0^x \frac{2b(y)}{\sigma^2} dy\right| \leq 2C\sigma^{-2} \left(1+A\right)A =: c_1(C,A,\sigma)\]
and consequently for $x\in [-A,A]$,
\[ \inf_{b\in\Sigma(C,A,\gamma,\sigma)} \exp\left( \int_0^x \frac{2b(y)}{\sigma^2} dy\right) \geq e^{ -c_1(C,A,\sigma)}.\]
Next, we bound $\sup_{b\in\Sigma(C,A,\gamma,\sigma)} C_{b,\sigma}$ from above by a constant not depending on $b$ and then the claim follows by combining those two bounds. Using the same bound as above, we have
\begin{align}\label{eqp: A2}
\int_{-A}^A \exp\left( \int_0^x \frac{2b(y)}{\sigma^2} dy\right) dx \leq 2A c_1(C,A,\sigma).
\end{align} 
Outside the interval $[-A,A]$ we use the condition $\sigma^{-2}b(x)\textrm{sign}(x)\leq -\gamma$ and get
\begin{align*}
\int_{-\infty}^{-A} \exp\left( \int_0^x \frac{2b(y)}{\sigma^2} dy\right) dx &= \int_{-\infty}^{-A}  \exp\left( -\int_{-A}^0 \frac{2b(y)}{\sigma^2} dy - \int_x^{-A} \frac{2b(y)}{\sigma^2} dy\right) dx \\
&\leq e^{c_1(C,A,\sigma)} \int_{-\infty}^{-A} e^{-2\gamma(-A-x)} dx\\
&=  e^{c_1(C,A,\sigma)} \left[ \frac{1}{2\gamma} e^{2\gamma(A+x)}\right]_{-\infty}^{-A} \\
&= \frac{1}{2\gamma} e^{c_1(C,A,\sigma)}.
\end{align*}
By the same arguments, 
\[ \int_A^\infty \exp\left( \int_0^x \frac{2b(y)}{\sigma^2} dy\right) dx \leq \frac{1}{2\gamma}e^{c_1(C,A,\sigma)}. \]
Putting all this together, 
\begin{align}\label{eqp: A3}
\begin{split}
\sup_{b\in\Sigma(C,A,\gamma,\sigma)}  C_{b,\sigma} &= \sup_{b\in\Sigma(C,A,\gamma,\sigma)} \int_{-\infty}^\infty \exp\left( \int_0^x 2\sigma^{-2}b(y) dy\right) dx\\
&\leq 2A c_1(C,A,\sigma) + \frac{1}{\gamma} e^{c_1(C,A,\sigma)}
\end{split}
\end{align} 
and the claim of the lemma follows with 
\[ L_* :=  e^{-c_1(C,A,\sigma)} \left(2A c_1(C,A,\sigma) + \frac{1}{\gamma} e^{c_1(C,A,\sigma)}\right)^{-1}. \]
\end{proof}

\begin{proof}[Proof of Corollary \ref{conv_emprical_density_uniform}]
Using Markov's inequality and Proposition~\ref{moments_local-invariant}, we directly get
\begin{align*}
&\sup_{b\in\Sigma(C,A,\gamma,\sigma)} \Pr_b\left( 
 \left\| \frac{1}{\sigma^2 T} L_T^z (X) - q_b(z)\right\|_\infty >\epsilon\right) \\
&\hspace{2cm}\leq \sup_{b\in\Sigma(C,A,\gamma,\sigma)}\frac{\E_b\left[ \left\| \frac{1}{\sigma^2 T} L_T^z (X) - q_b(z)\right\|_\infty\right]}{\epsilon}\\
&\hspace{2cm}\leq \frac{c_1}{\epsilon}\left( \frac1T + \frac{1}{\sqrt{T}}\left( 2+\sqrt{\log T}\right) + Te^{-c_2T}\right) \longrightarrow 0.
\end{align*}
\end{proof}

\begin{proof}[Proof of Proposition \ref{uniform_ergodic}]
By the occupation times formula~\ref{occupation_times_formula},
\begin{align*}
&\sup_{b\in\Sigma(C,A,\gamma,\sigma)}\Pr_b\left(\sup_{f\in\mathcal{F}} \left|\frac1T \int_0^T f(X_s) ds - \int_\R f(z) q_b(z) dz \right| >\epsilon\right)\\
&\hspace{1cm} =  \sup_{b\in\Sigma(C,A,\gamma,\sigma)}\Pr_b\left( \sup_{f\in\mathcal{F}}\left|\int_\R f(z) \left( \frac{1}{\sigma^2 T}L_T^z(X) -q_b(z)\right) dz \right| >\epsilon\right) \\
&\hspace{1cm} \leq \sup_{b\in\Sigma(C,A,\gamma,\sigma)}\Pr_b\left(  \left\| \frac{1}{\sigma^2 T}L_T^\cdot(X) -q_b\right\|_{[-A,A]}\ \sup_{f\in\mathcal{F}}\int_\R |f(z)| dz  >\epsilon\right) \\
&\hspace{1cm} \leq \sup_{b\in\Sigma(C,A,\gamma,\sigma)}\Pr_b\left(  \left\| \frac{1}{\sigma^2 T}L_T^\cdot (X) -q_b\right\|_{[-A,A]}  >\frac{\epsilon}{2A C_\mathcal{F}}\right),
\end{align*}
where we used that by assumption $\int_\R |f(z)|dz \leq 2A C_{\mathcal{F}}$ uniformly in $f\in\mathcal{F}$. Now, the last probability converges to zero for $T\to\infty$ due to Corollary~\ref{conv_emprical_density_uniform} and the claim follows.
\end{proof}

\begin{proof}[Proof of Lemma \ref{lemma_b+eta}]
With $b_0 \in \textrm{Lip}_\textrm{loc}(\R)$, we have $b_0\pm\eta\in \textrm{Lip}_\textrm{loc}(\R)$. Next, 
\begin{align*}
|b_0(x)\pm\eta| \leq |b_0(x)| + \eta \leq \left(\frac{C}{2} -\eta\right) (1+|x|) + \eta \leq \frac{C}{2}(1+|x|).
\end{align*}
Finally, for $|x|\geq A$, we have $\sigma^{-2}b_0(x)\textrm{sign}(x)\leq -(\gamma+\frac{\eta}{\sigma^2})$ and hence for those $x$,
\begin{align*}
\sigma^{-2}(b_0(x)\pm\eta)\textrm{sign}(x) &= \sigma^{-2}b_0(x)\textrm{sign}(x) \pm\sigma^{-2}\textrm{sign}(x)\eta \\
&\leq -\gamma - \sigma^{-2}\eta +\sigma^{-2}\eta = -\gamma.
\end{align*} 
\end{proof}

\subsection{Generalization of Proposition \ref{moments_local-invariant}}\label{A3_SubSec}

In this subsection we will generalize Proposition $\ref{moments_local-invariant}$ to diffusions that are not started in the invariant distribution. To this aim we consider a diffusion $X^{x_0} = (X_t^{x_0})_{t\geq 0}$ solving
\[ dX_t^{x_0} = b(X_t^{x_0}) dt + \sigma dW_t, \quad X_0^{x_0}= x_0, \]
for some fixed initial value $x_0\in [-A,A]$. We denote by $\xi$ a random variable that is distributed under the invariant law $\mu_b$ as in the preceeding subsections. Furthermore, we set $\tilde{G}:= \sup_{b\in\Sigma(C,A,\gamma,\sigma)} C_{b,\sigma^2}$ which is finite as seen in \eqref{eqp: A3} and define
\begin{align}\label{eqp: constant_G}
G:= 2\tilde G \sup_{b\in\Sigma(C,A,\gamma,\sigma)} \int_{-A}^A \exp\left( -\int_0^x 2\sigma^{-2} b(u) du \right) dx, 
\end{align} 
where we see that the integral is uniformly bounded over $b\in\Sigma(C,A,\gamma,\sigma)$ in the same way as in \eqref{eqp: A2}.\\
For the proof of Proposition~\ref{moments_local-invariant}, the stationarity assumption is used in the form of the moment bound
\[ \E_b\left[ |X_t|^p\right] = \E_b\left[ |\xi|^p\right] \leq c_{mo}^p p^p \]
for some constant $c_{mo}\geq 0$, see Lemma~$17$ in \cite{Strauch}. In order to derive the result for $X^{x_0}$, we first show that a moment inequality of the form 
\[ \E_b\left[ |X_t^{x_0}|^p\right] \leq \C_{mo}^p p^p \]
holds for a different constant $\C_{mo}>0$, see Lemma~\ref{lemma_C_mo}. Then the result of Proposition~\ref{moments_local-invariant} can be transferred to $X^{x_0}$ as this result only uses the order $p^p$ of the moment bound which is the same for $X_0=x_0$ and $X_0=\xi\sim\mu_b$. This is described in detail at the end of the subsection.

\begin{lemma}\label{lemma_E_ergodic}
Let $f:\R\rightarrow\R$ be a measurable function and $\xi\sim\mu_b$. Then for the constant $G$ given in \eqref{eqp: constant_G}, we have
\[ \left| \E_b\left[ \int_0^T f(X_t^{x_0}) dt\right] - T\E_b\left[ f(\xi)\right]\right| \leq G\E_b\left[ |f(\xi)|\right]. \]
\end{lemma}
\begin{proof}
We know that the claim is true for $f\geq 0$, which was shown in Lemma $3.4.8$ in \cite{Kutoyants2}. It is important to note that we used the exact constant in equation $(4.21)$ in the reference, by which 
\[ \E_b[\tau]\leq 2(a-c)\tilde G = 2 \tilde G\int_{-A}^A \exp\left( -\int_0^x 2\sigma^{-2} b(u) du\right) dx\]
in the proof of Lemma~$3.4.8$, where this upper bound of $\E_b[\tau]$ was used and yields the constant $G$ within the claim.\\
For the general case, we split $f$ into its positive and negative part, i.e. $f = f^+ - f^-$. As $f^+, f^-\geq 0$, we get
\begin{align*}
&\left| \E_b\left[ \int_0^T f(X_t^{x_0}) dt\right] - T\E_b\left[ f(\xi)\right]\right| \\
&\hspace{1cm} = \left| \E_b\left[ \int_0^T f^+(X_t^{x_0}) - f^-(X_t^{x_0}) dt\right] - T\E_b\left[ f^+(\xi) - f^-(\xi)\right]\right|  \\
&\hspace{1cm} \leq \left| \E_b\left[ \int_0^T f^+(X_t^{x_0}) dt\right] - T\E_b\left[ f^+(\xi)\right]\right|\\
&\hspace{3cm} + \left| \E_b\left[ \int_0^T f^-(X_t^{x_0}) dt\right] - T\E_b\left[ f^-(\xi)\right]\right| \\
&\hspace{1cm} \leq G\E_b\left[ f^+(\xi)\right] + G\E_b\left[ f^-(\xi)\right] \\
&\hspace{1cm} = G\E_b\left[ |f(\xi)|\right].
\end{align*}
\end{proof}

We assume the following lemma to be commonly known, but as we did not find a reference for it, a proof is given.

\begin{lemma}\label{lemma_derivative}
For the absolute value function $|\cdot|:\R\rightarrow\R$ the following holds true:
\begin{enumerate}
\item[(i)] The function $x|x|$ is continuously differentiable.
\item[(ii)] For $n$ odd and $n\geq 3$, the function $|x|^n$ is twice continuously differentiable with
\begin{align*}
\frac{d}{dx} |x|^n = nx|x|^{n-2}, \quad \textrm{ and }\quad 
\frac{d^2}{dx^2} |x|^n = n(n-1)|x|^{n-2}.
\end{align*}
\end{enumerate}
\end{lemma}
\begin{proof}
\begin{enumerate}
\item[(i)] It is clear that $x|x|$ is differentiable for $x\neq 0$ with
\begin{align*}
\frac{d}{dx} (x|x|) = \begin{cases}
2x & \textrm{ for } x>0, \\
-2x & \textrm{ for } x<0.
\end{cases}
\end{align*}  
For $x=0$, the left- and right-hand limits of the difference quotient have to be identical. This is the case, as
\[ \lim_{h\searrow 0} \frac{h(-h)}{h} = 0 = \lim_{h\nearrow 0}\frac{h^2}{h}.\]
In particular, we see that the derivative is continuous in $x=0$.

\item[(ii)] This follows by usual differentiation rules and the fact that $\frac{d}{dx}|x|=\frac{x}{|x|}$ for $x\neq 0$. In $x=0$ we consider the limit of the difference quotient as in (i), which exists and equals zero.
\end{enumerate}
\end{proof}

\begin{lemma}\label{lemma_E=0}
Let $\xi\sim \mu_b$. Then for $n\geq 2$,
\[ n\E_b\left[ |\xi|^{n-2}\xi b(\xi)\right] + \frac{n(n-1)}{2} \sigma^2 \E_b\left[ |\xi|^{n-2}\right] = 0.\]
\end{lemma}
\begin{proof}
The function $|x|^{n-2}x$ is differentiable with derivative
\begin{align*}
\frac{d}{dx}\left( |x|^{n-2}x\right) &= |x|^{n-2} + x (n-2) |x|^{n-3}\frac{x}{|x|}\\
&= |x|^{n-2} + (n-2) |x|^{n-3} \frac{|x|^2}{|x|}\\
&= (n-1)|x|^{n-2}.
\end{align*}
This is clear for $n$ even and can be seen by Lemma~\ref{lemma_derivative} otherwise. By the relation $q_b'(x) = 2\sigma^{-2}b(x)q_b(x)$ and partial integration,
\begin{align*}
n\E_b\left[ |\xi|^{n-2}\xi b(\xi)\right]  &= n\int_\R |x|^{n-2}x b(x) q_b(x) dx\\
&= \frac{n\sigma^2}{2} \int_\R  x|x|^{n-2} q_b'(x) dx \\
&= \frac{n\sigma^2}{2}\left( \left[ x|x|^{n-2}q_b(x)\right]_{-\infty}^\infty - \int_\R (n-1)|x|^{n-2} q_b(x) dx\right) \\
&= -\frac{\sigma^2}{2} n(n-1) \E_b\left[ |\xi|^{n-2}\right].
\end{align*}
In the last step we used that $\lim_{x\to\pm\infty} x|x|^{n-2}q_b(x) =0$, which follows from the fact that by \eqref{eqp: A1} for some constant $\tilde c$, 
\begin{align*}
q_b(x) &= \frac{1}{C_{b,\sigma}\sigma^2} \exp\left( \int_0^x \frac{2b(y)}{\sigma^2} dy\right)\\
& \leq \frac{1}{C_{b,\sigma}\sigma^2} \exp\left( \tilde c -2\gamma (|x|-A)_+\right). 
\end{align*} 
\end{proof}

\begin{lemma}\label{lemma_C_mo}
There exists a constant $\C_{mo}>0$ such that for all $p\geq 1$,
\[ \E_b\left[ |X_t^{x_0}|^p\right]^\frac1p \leq \C_{mo} p \quad \textrm{ for all } t\geq 0.\]
\end{lemma}
\begin{proof}
First, let $p\geq 2$. Then we have by the It\^{o} formula and Lemma~\ref{lemma_derivative},
\begin{align*}
|X_t^{x_0}|^p &= |x_0|^p + p \int_0^t X_s^{x_0} |X_s^{x_0}|^{p-2} dX_s^{x_0} + \frac{p(p-1)}{2}\int_0^t |X_s^{x_0}|^{p-2} d\langle X^{x_0}\rangle_s \\
&= |x_0|^p + p\sigma \int_0^t X_s^{x_0} |X_s^{x_0}|^{p-2} dW_s + p\int_0^t X_s^{x_0}|X_s^{x_0}|^{p-2} b(X_s^{x_0}) ds\\
&\hspace{2cm} + \frac{p(p-1)}{2}\int_0^t \sigma^2 |X_s^{x_0}|^{p-2} ds.
\end{align*}
Consequently, the following is true for the expectation, where we apply Lemma~\ref{lemma_E=0} for adding zero in the second step and Lemma~\ref{lemma_E_ergodic} in the last one: \vspace{0.2cm}
\begin{align*}
&\E_b\left[|X_t^{x_0}|^p\right] \\
&\hspace{0.1cm}= |x_0|^p + p \E_b\left[ \int_0^t X_s^{x_0}|X_s^{x_0}|^{p-2} b(X_s^{x_0}) ds\right] + \frac{p(p-1)}{2} \E_b\left[ \int_0^t \sigma^2 |X_s^{x_0}|^{p-2} ds\right] \\
&\hspace{0.1cm}= |x_0|^p - t\left( p\E_b\left[ |\xi|^{p-2}\xi b(\xi)\right] + \frac{p(p-1)}{2}\E_b\left[ \sigma^2 |\xi|^{p-2}\right]\right) \\
&\hspace{1cm} +  p \E_b\left[ \int_0^t X_s^{x_0}|X_s^{x_0}|^{p-2} b(X_s^{x_0}) ds\right] + \frac{p(p-1)}{2} \E_b\left[ \int_0^t \sigma^2 |X_s^{x_0}|^{p-2} ds\right]  \\
&\hspace{0.1cm}\leq  |x_0|^p + p\left| \E_b\left[ \int_0^t X_s^{x_0}|X_s^{x_0}|^{p-2} b(X_s^{x_0}) ds \right] - t\E_b\left[ |\xi|^{p-2}\xi b(\xi)\right]\right| \\
&\hspace{1cm} + \frac{p(p-1)}{2}\left| \E_b\left[\int_0^t \sigma^2 |X_s^{x_0}|^{p-2}ds\right] - t\E_b\left[ \sigma^2|\xi|^{p-2}\right]\right|\\
&\hspace{0.1cm}\leq |x_0|^p + pG \E_b\left[ |\xi^{p-1} b(\xi)|\right] + \frac{p(p-1)}{2} G\E_b\left[ \sigma^2 |\xi|^{p-2}\right].
\end{align*}
Using the $L^p(\Pr_b)$-bound of $\xi$ from Lemma $17$ in \cite{Strauch}, there exists a constant $c_{mo}\geq 1$ independent of $b$ such that
\[ \E_b\left[\sigma^2 |\xi|^{p-2}\right] \leq  c_{mo}^{p-2}\sigma^2 (p-2)^{p-2}.\]
By the at most linear growth condition and the same lemma, we may further conclude
\begin{align*}
\E_b\left[ |\xi^{p-1} b(\xi)|\right] &\leq \E_b\left[ |\xi|^{p-1} C(1+|\xi|)\right] \\
&= C\E_b\left[ |\xi|^{p-1} + |\xi|^p\right] \\
&\leq C \left( c_{mo}^{p-1} (p-1)^{p-1} + c_{mo}^p p^p\right) \\
&\leq 2C c_{mo}^p p^p.
\end{align*} 
In consequence, 
\begin{align*}
\E_b\left[ |X_t^{x_0}|^p\right] &\leq |x_0|^p + p2Cc_{mo}^p p^p G + G\frac{p(p-1)}{2} \sigma^2 c_{mo}^{p-2} (p-2)^{p-2} \\
&\leq |x_0|^p + 2CG c_{mo}^p p^{p+1} + \frac12 G\sigma^2 c_{mo}^{p-2} p^p \\
&\leq |x_0|^p + p^{p+1}  G c_{mo}^p \left( 2C + \sigma^2 2^{-1}c_{mo}^{-2}\right).
\end{align*}
Now using $(a^p+b^p)^\frac1p \leq a+b$ for $a,b\geq 0$, $|x_0|\leq A$ and $p^\frac1p \leq 2$, we arrive at
\begin{align*}
\E_b\left[ |X_t^{x_0}|^p\right]^\frac1p &\leq \left(  |x_0|^p + p^{p+1}  G c_{mo}^p \left( 2C + \sigma^2 2^{-1}c_{mo}^{-2}\right) \right)^\frac1p \\
&\leq |x_0| + p^{1+1/p} c_{mo} \left( 2GC + G\sigma^2 2^{-1}c_{mo}^{-2}\right)^\frac1p \\\
&\leq |x_0| + 2p c_{mo}\max\left\{ \left( 2GC + G\sigma^2 2^{-1}c_{mo}^{-2}\right),1\right\} \\
&\leq p\left( A + 2c_{mo}\max\left\{ \left( 2GC + G\sigma^2 2^{-1}c_{mo}^{-2}\right),1\right\} \right).
\end{align*}
Thus, we have the desired inequality $\E_b\left[|X_t^{x_0}|^p\right]^\frac1p\leq \C_{mo}' p$ for all $p\geq 2$ and $\C_{mo}' = A + 2c_{mo}\max\left\{ \left( 2GC + G\sigma^2 2^{-1}c_{mo}^{-2}\right),1\right\} $. For $1\leq p<2$, 
\[ \E_b\left[ |X_t^{x_0}|^p\right] \leq \E_b\left[ |X_t^{x_0}|^{2p}\right]^\frac12 \leq \sqrt{ (\C_{mo}')^{2p} (2p)^{2p}} \leq (2\C_{mo}')^p p^p\]
and consequently $\E_b\left[ |X_t^{x_0}|^p\right]^\frac1p \leq 2\C_{mo}' p$. Combining both cases for the value of $p$, we arrive at the claim by setting $\C_{mo} = 2\C_{mo}'$.
\end{proof}

We now turn to the necessary modifications in the proofs of \cite{Strauch} to adapt them to the case of the diffusion $X^{x_0}$ that is not started in the invariant law but at a fixed point $x_0$. The following numbers of sections and results refer to those in \cite{Strauch}. We first remark that the results of Section~$2$ and $3$ in this paper are formulated in a general setting of continuous semimartingales, which means nothing has to be adapted to our setting here.

\begin{enumerate}
\item[(1)] First, we check Assumption~$1$. As our diffusion coefficient is constant, the function $\phi_2(t) := \sigma\sqrt{t}$ can be used for the same reason as in the stationary case considered in the paper. With the at most linear growth condition on $b$ and Lemma~$3.4.8$ in \cite{Kutoyants2},
\begin{align*}
&\|x_0\|_{L^p(\Pr_b)} + \left\| \int_0^t |b(X_s^{x_0})|ds\right\|_{L^p(\Pr_b)}\\
&\hspace{1.5cm}\leq |x_0| + C\E_b\left[  t^p\left( \frac{1}{t} \int_0^t 1+|X_s^{x_0}| ds \right)^p\right]^\frac1p \\
&\hspace{1.5cm}\leq |x_0| + Ct \E_b\left[ \frac1t \int_0^t (1+|X_s^{x_0}|)^p ds \right]^\frac1p\\
&\hspace{1.5cm}\leq |x_0| + C t^{1-1/p} \left( (t+G) \E_b\left[ (1+|\xi|)^p\right]\right)^\frac1p\\
&\hspace{1.5cm}\leq |x_0| + 2C t (1+G)\left(1+c_{mo}p\right)
\end{align*} 
for the constant $c_{mo}$ from Lemma~$17$ in \cite{Strauch} that is independent of $b$. Hence, we may choose $\phi_1$ as
\[ \phi_1(t) := \max\left\{ |x_0| + 2C(1+G)(1+c_{mo}), \sigma^2\right\} t,\]
where the maximum ensures that $\phi_2(t)\leq \sqrt{\phi_1(t)}$.

\item[(2)] Corollary~$6$ directly transfers to $X^{x_0}$ as it only uses results from Section~$2$ and the validity of Assumption~$1$ that was checked in (1).

\item[(3)] Next, we check Proposition~$7$. The first step where stationarity is needed is from (D.3) to (D.4). By Jensen's inequality  and Lemma~$3.4.8$ in \cite{Kutoyants2} we get for $p\geq 2$,
\begin{align*}
t^{-p/2} \E_b\left[ \left(\int_0^t (1+X_s^{x_0})^{2\eta}) ds\right)^\frac{p}{2}\right] &\leq \E_b\left[ \frac1t \int_0^t (1+|X_s^{x_0}|)^{p\eta} ds\right] \\
&\leq (1+G) \E_b\left[ (1+|\xi|)^{p\eta}\right] \\
&\leq (1+G) 2^{p\eta}\left(1+(c_{mo} p\eta)^{p\eta}\right) \\
&\leq p^{p\eta} (1+G) 2^{p\eta}\left(1+(c_{mo} \eta)^{p\eta}\right),
\end{align*}
where we used in the third step that $\E_b[|\xi|^p]\leq (c_{mo}p)^p$ from Lemma~$17$ in \cite{Strauch}.\\
The inequality for $1\leq p<2$ can be modified in the same way. Then the moment bound of $|\mathbb{M}_t^f|$ follows with an additional factor $2^{\eta+1/2}(1+G)$, but the same exponent of $p$.\\
Bounding the remainder term $\R_t^f$ follows the same lines as in the original proof and leads to the upper bound 
\[ \mathcal{S} \overline{\Lambda}_{\textrm{prox}}\left( x_0 +\frac{1}{\eta+1} x_0^{\eta+1} + \|X_t^{x_0}\|_{L^p(\Pr_b)} + \frac{1}{\eta+1}\|X_t^{x_0}\|_{L^p(\Pr_b)}\right). \]
Now, we use the $L^p(\Pr_b)$-bound of Lemma~\ref{lemma_C_mo} instead of the moment bound $c_{mo}p$ of Lemma~$17$ in \cite{Strauch} and have the same upper bound as in the paper concerning the order of $p$ and $\mathcal{S}$, but with modified constant. \\
The estimates for $\mathbb{M}_t^{b_0}$ and $\R_t^{b_0}$ in the second part of the proof where $f=b_0$ can be modified in the same way.

\item[(4)] The proof of Theorem~$9$ can be completely transfered, one just has to change the constants as Proposition~$7$ is used. Note however, that the important exponents of $p$ and $\mathcal{S}$ did not have changed there. 

\item[(5)] The proof of Theorem~$10$ carries over (with modified constants) as it only uses Corollary~$6$ and Proposition~$7$ which are both available as seen in (2) and (3) with modified constants. The important dependence on $p$ remains the same as this was the case in both other results.

\item[(6)] Corollary~$12$ is a consequence of Theorem~$9$ and thus still valid with modified constants, see (4).

\item[(7)] Most of the proof of Theorem~$13$ does not take into account the distribution of $X_0$. Just in the final steps where Proposition~$7$ and Theorem~$10$ are applied, we have to take their (modified) constants. Furthermore, as $X_0$ is not distributed under the invariant measure, we have to substitute it by $\xi$ in the deviation expression
\[ \sup_{b\in\Sigma} \Pr_b\left( \left\| \sqrt{t} \left( \frac1t \int_0^t f(X_s) dX_s - \E_b[f(\xi) b(\xi)]\right) \right\|_{\mathcal{F}_{K,h}} \geq \phi(u)\right) \leq e^{-u}.\]

\item[(8)] The proof of Corollary~$14$, which is our desired moment estimate of the deviation of the local time from the invariant density (Proposition~\ref{moments_local-invariant}), carries over from Corollary~$12$ and Theorem~$13$.
\end{enumerate}
