# Supplementary material for: Sharp adaptive and pathwise stable similarity testing for scalar ergodic diffusions
Source: arXiv:2203.13776 source file (2024-04-16)
Supplement: Supplementary file 12 [file Multiscale_Testing+Supplement.tex]

% Template for the submission to:
%   The Annals of Probability           [aop]
%   The Annals of Applied Probability   [aap]
%   The Annals of Statistics            [aos] 
%   The Annals of Applied Statistics    [aoas]
%   Stochastic Systems                  [ssy]
%
%Author: In this template, the places where you need to add information
%        (or delete line) are indicated by {???}.  Mostly the information
%        required is obvious, but some explanations are given in lines starting
%Author:
%All other lines should be ignored.  After editing, there should be
%no instances of ??? after this line.

% use option [preprint] to remove info line at bottom
% journal options: aop,aap,aos,aoas,ssy
% natbib option: authoryear
\pdfoutput=1

\documentclass[aos, preprint]{imsart}

\RequirePackage[OT1]{fontenc}
\RequirePackage{graphicx,color,amssymb,amsmath,amsthm,mathrsfs}
\RequirePackage[numbers]{natbib}
\RequirePackage[colorlinks,citecolor=blue,urlcolor=blue, hypertexnames=false]{hyperref}
\RequirePackage{tikz}
\RequirePackage{bbm}
\RequirePackage{algpseudocode}
\RequirePackage{algorithm2e}
\usepackage{caption} 
\usepackage{xr}
\usepackage{ulem} % Zum Durchstreichen verwendet
\usepackage{tabu}
\usepackage{float}
\usepackage{flowchart}
\usetikzlibrary{arrows}

\floatstyle{plaintop}
\restylefloat{table}
\captionsetup[table]{singlelinecheck=false}



\allowdisplaybreaks




%\usepackage{amsthm,amsmath,natbib}
%\RequirePackage[colorlinks,citecolor=blue,urlcolor=blue]{hyperref}

% provide arXiv number if available:
%\arxiv{arXiv:0000.0000}

% put your definitions there:
\startlocaldefs
%\numberwithin{equation}{section}
%\theoremstyle{plain}
\newtheorem{definition}{Definition}[section]
\newtheorem{thm}[definition]{Theorem}
\newtheorem{lemma}[definition]{Lemma}
\newtheorem{proposition}[definition]{Proposition}
\newtheorem{cor}[definition]{Corollary}
\newtheorem{prop}[definition]{Proposition}
\newtheorem{remark}[definition]{Remark}

\renewcommand{\theequation}{\thesection.\arabic{equation}}

\def\R{\mathbb{R}}
\def\C{\mathbb{C}}
\def\N{\mathbb{N}}
\def\Q{\mathbb{Q}}
\def\Z{\mathbb{Z}}

\def\1{\mathbbm{1}}

\def\E{\mathbb{E}}
\def\Pr{\mathbb{P}}
\endlocaldefs




\makeatletter
\renewcommand\tableofcontents{%
    \@starttoc{toc}%
}
\makeatother



\makeatletter
\def\eqref{\@ifstar\@eqref\@@eqref}
\def\@eqref#1{\textup{\tagform@{\ref*{#1}}}}
\def\@@eqref#1{\textup{\tagform@{\ref{#1}}}}
\makeatother 



%\externaldocument[]{Supplement}


\begin{document}

\begin{frontmatter}

% "Title of the paper"
\title{Sharp adaptive and pathwise stable similarity testing for scalar ergodic diffusions}
\runtitle{Similarity testing for ergodic diffusions}

% indicate corresponding author with \corref{}
% \author{\fnms{John} \snm{Smith}\corref{}\ead[label=e1]{smith@foo.com}\thanksref{t1}}
% \thankstext{t1}{Thanks to somebody} 
%\address{Institute of Mathematics\\ Ernst-Zermelo-Straße 1\\ 79104 Freiburg\\ Germany\\ printead{e1}}
%\affiliation{Albert-Ludwigs-Universität Freiburg}

\author{\fnms{Johannes} \snm{Brutsche}\ead[label=e1]{johannes.brutsche@stochastik.uni-freiburg.de}}
%\address{\printead{e1}}
\and
\author{\fnms{Angelika} \snm{Rohde}\ead[label=e2]{angelika.rohde@stochastik.uni-freiburg.de}}
%\address{\printead{e2}}
%\affiliation{???}

%\thankstext{T1}{Supported by the ANR Grant Labex Ecodec (ANR-11-LABEX-0047).}

\begin{aug}
%%%%%%%%%%%%%%%%%%%%%%%%%%%%%%%%%%%%%%%%%%%%%%%
%% Only one address is permitted per author. %%
%% Only division, organization and e-mail is %%
%% included in the address.                  %%
%% Additional information can be included in %%
%% the Acknowledgments section if necessary. %%
%%%%%%%%%%%%%%%%%%%%%%%%%%%%%%%%%%%%%%%%%%%%%%%
%\author{\fnms{Johannes} \snm{Brutsche}\ead[label=e1]{johannes.brutsche@stochastik.uni-freiburg.de}}
%\and
%\author{\fnms{Angelika} \snm{Rohde}\ead[label=e2]{angelika.rohde@stochastik.uni-freiburg.de}}
%\affiliation{University of Freiburg}
%%%%%%%%%%%%%%%%%%%%%%%%%%%%%%%%%%%%%%%%%%%%%%
%% Addresses                                %%
%%%%%%%%%%%%%%%%%%%%%%%%%%%%%%%%%%%%%%%%%%%%%%
%\address{Institute of Mathematics\\ Ernst-Zermelo-Straße 1\\ 79104 Freiburg\\ Germany \\ \printead{e1,e2}}
%\address{Institute of Mathematics\\ Ernst-Zermelo-Straße 1\\ 79104 Freiburg\\ Germany \\ \printead{e2}}
\end{aug}



\runauthor{J. Brutsche and A. Rohde}

\affiliation{Albert-Ludwigs-Universit\"at Freiburg}



\begin{abstract}
Within the nonparametric diffusion model, we develop a multiple test to infer about \textit{similarity} of an unknown drift $b$ 
to some reference drift $b_0$: At prescribed significance, we simultaneously identify those regions where violation from similarity occurs, without a priori knowledge of their number, size and location. This test is shown to be minimax-optimal and adaptive. At the same time, the procedure is robust under small deviation from Brownian motion as the driving noise process. A detailed investigation for fractional driving noise, which is neither a semimartingale nor a Markov process, is provided for Hurst indices close to the Brownian motion case.
\end{abstract}

\begin{keyword}[class=MSC]
\kwd[Primary ]{62G10}
\kwd{62G20}
\kwd{62M02}
\kwd[; secondary ]{60G22}
\end{keyword}

\begin{keyword}
\kwd{Similarity}
\kwd{sharp adaptivity}
\kwd{empirical processes}
\kwd{diffusions}
\end{keyword}


\end{frontmatter}


% AOS,AOAS: If there are supplements please fill:
%\begin{supplement}[id=suppA]
%  \sname{Supplement A}
%  \stitle{Title}
%  \slink[doi]{10.1214/00-AOASXXXXSUPP}
%  \sdatatype{.pdf}" 
%  \sdescription{Some text}
%\end{supplement}




\numberwithin{equation}{section}
\addtocontents{toc}{\protect\setcounter{tocdepth}{0}}

\input{Sections/Introduction}
\input{Sections/Preliminaries}
\input{Sections/Simple_null}
\input{Sections/Multiscale_Test}
\input{Sections/Power_considerations}
\input{Sections/Stability}
%\input{Sections/Implementation}
\input{Sections/weak}
\input{Sections/Further_results}
\input{Sections/Outlook}


\smallskip
\textbf{Acknowledgments.} We are very grateful to two anonymous referees for two constructive and detailed reports even on the whole supplementary material which led to a significant clarification of our presentation.

\smallskip
\textbf{Funding.} This work has been supported in part by the \textit{Research Unit~$5381$}, DFG Research Grant RO 3766/8-1 and the CRC 1597.



\begin{thebibliography}{9}

\bibitem{Strauch}
\textsc{Aeckerle-Willems, C. and Strauch, C.} (2021). 
Concentration of scalar ergodic diffusions and some statistical implications. \textit{Ann. Inst. H. Poincaré Probab. Statist.}
\textbf{57}(4) 1857–-1887.
\MR{4328556}


%\bibitem{Ait}
%\textsc{A\"{i}t-Sahalia, Y. and Mancini, L.} (2008). 
%Out of sample forecasts of quadratic variation. \textit{Journal of Econometrics}
%\textbf{147} 17–-33.
%\MR{2472978}


\bibitem{Aliprantis}
\textsc{Aliprantis, C. D. and Border, K. C.} (1994). \textit{Infinite Dimensional Analysis}, Studies in Economic Theory 4, Springer-Verlag, Berlin.
\MR{1321140}


\bibitem{Altman}
\textsc{Altman, C.G. and Bland, J.M.} (1995). 
Statistics notes: Absence of evidence is not evidence of absence. \textit{British Medical Journal}
\textbf{311}(7003) 485.%–-??.
%\MR{4328556}


\bibitem{Anderson/Kurtz}
\textsc{Anderson, D.F. and Kurtz, T.G.} (2015). \textit{Stochastic Analysis of Biochemical Systems},  Mathematical Biosciences Institute Lecture Series 1.2,
ChamMBI Mathematical Biosciences Institute, Ohio State University, Columbus, OH.
\MR{3363610}


\bibitem{Bai}
\textsc{Bai, L. and Ma, J.} (2015). 
Stochastic differential equations driven by fractional Brownian motion and Poisson point process. \textit{Bernoulli}
\textbf{21}(1) 303–-334.
\MR{3322320}


%\bibitem{Banon}
%\textsc{Banon, G.} (1978). 
%Nonparametric identification for diffusion processes. \textit{SIAM Journal on Control and Optimization}
%\textbf{16}(3) 380–-395.
%\MR{0492159}


\bibitem{Barlow/Yor}
\textsc{Barlow, M.T. and Yor, M.} (1982). 
Semimartingale inequalities via the Garsia-Rodemich-Rumsey lemma, and applications to local times. \textit{Journal of Functional Analysis}
\textbf{49}(2) 198–-229.
\MR{0680660}



\bibitem{Berkson}
\textsc{Berkson, J.} (1938)
Some difficulties of interpretation encountered in the application of the chi-square test. \textit{Journal of the American Statistical Association}
\textbf{33}(203) 526--536
%\MR{....}


\bibitem{Billingsley}
\textsc{Billingsley, P.} (1968). \textit{Convergence of probability measures}, John Wiley \& Sons, Inc., New York-London-Sydney.
\MR{0233396}


\bibitem{Brutsche}
\textsc{Brutsche, J.} (2022). \textit{Sharp adaptive similiarity testing with pathwise stability for ergodic diffusions}, PhD thesis, Albert-Ludwigs-Universität Freiburg.


\bibitem{Freitag}
\textsc{Busam, R. and Freitag, E.} (2009). \textit{Complex Analysis}, 2nd ed. Universitext. Springer, Berlin.
\MR{2513384}


\bibitem{Buecher}
\textsc{Bücher, A., Dette, H. and Heinrichs, F.} (2021).
Are deviations in a gradually varying mean relevant? A testing approach based on sup-norm estimators. \textit{The Annals of Statistics}
\textbf{49}(6) 3583--3617.
\MR{4352542}


\bibitem{CCK}
\textsc{Chernozhukov, V., Chetverikov, D. and Kato, K.} (2014). 
Gaussian approximation of suprema of empirical processes. \textit{Annals of Statistics}
\textbf{42}(4) 1564–-1597.
\MR{3262461}


\bibitem{Dalalyan}
\textsc{Dalalyan, A.} (2005). 
Sharp adaptive estimation of the drift function for ergodic diffusions. \textit{The Annals of Statistics}
\textbf{33}(5) 2507–-2528.
\MR{2253093}


\bibitem{Dalalyan/Reiss}
\textsc{Dalalyan, A. and Reiß, M.} (2006). 
Asymptotic statistical equivalence for scalar ergodic diffusions. \textit{Probab. Theory Related Fields}
\textbf{134}(2) 248–-282.
\MR{2222384}


\bibitem{Datta}
\textsc{Datta, P. and Sen, B. } (2021). 
Optimal inference with a multidimensional multiscale statistic. \textit{Electronic Journal of Statistics}
\textbf{15}(2) 5203–-5244.
\MR{4349258}


\bibitem{Decreusefond}
\textsc{Decreusefond, L. and Üstünel, A.S.} (1999).
Stochastic Analysis of the Fractional Brownian Motion. \textit{Potential Analysis}
\textbf{10}(2) 177--214.
\MR{1677455}


%\bibitem{Dette1}
%\textsc{Dette, H. and Wied, D.} (2016).
%Detecting relevant changes in time series models. \textit{Journal of the Royal Statistical Society. Series B. Statistical Methodology}
%\textbf{78}(2) 371--394.
%\MR{3454201}


\bibitem{Dette}
\textsc{Dette, H., Kokot, K. and Aue, A.} (2020).
Functional data analysis in the Banach space of continuous functions. \textit{The Annals of Statistics}
\textbf{48}(2) 1168--1192.
\MR{4102692}


\bibitem{Diehl/Friz}
\textsc{Diehl, J., Friz, P. and Mai, H.} (2016). 
Pathwise stability of likelihood estimators for diffusions via rough paths. \textit{The Annals of Applied Probability}
\textbf{16}(4) 2169–-2192.
\MR{3543893}


\bibitem{Donoho}
\textsc{Donoho, D.L.} (1994).
Statistical estimation and optimal recovery. \textit{The Annals of Statistics}
\textbf{22} 238--270.
\MR{1272082}


\bibitem{Walther}
\textsc{Dümbgen, L. and Walther, G.} (2008).
Multiscale inference about a density. \textit{The Annals of Statistics}
\textbf{36}(4) 1758--1785; 
accompanying technical report, version 2. Available at \url{http://arxiv.org/abs/0706.3968}
%\textit{University of Bern - Forschungsbericht 56}
%\textbf{3} 231--283.
\MR{2435455}


\bibitem{Duembgen/Spokoiny}
\textsc{Dümbgen, L. and Spokoiny, V.G.} (2001).
Multiscale testing of qualitative hypotheses. \textit{The Annals of Statistics}
\textbf{29}(1) 124--152.
\MR{1833961}


\bibitem{Piterbarg}
\textsc{Dümbgen, L., Piterbarg, V.I. and Zholud, D.} (2006). 
On the limit distribution of multiscale test statistics for nonparametric curve estimation. \textit{Mathematical Methods of Statistics}
\textbf{15}(1) 20–-25.
\MR{2225428}


%\bibitem{Durrett}
%\textsc{Durrett, R.} (1996). \textit{Stochastic calculus - A practical introduction}, Probability and Stochastic Series,
%CRC Press, Boca Raton.
%\MR{1398879}


%\bibitem{Elstrodt}
%\textsc{Elstrodt, J.} (2005). \textit{Maß- und Integrationstheorie (Measure and integration theory)} 4th ed. Grundwissen Mathematik, 
%Springer, Berlin.
%\MR{2257838}


\bibitem{Erdelyi}
\textsc{Erdélyi, A., Magnus, W., Oberhettinger, F. and Tricomi, F.G.} (1981). \textit{Higher transcendental functions. Vol. I.}, Based on notes left by Harry Bateman. With a preface by Mina Rees. With a foreword by E. C. Watson. Reprint of the 1953 original.
Robert E. Krieger Publishing Co., Inc., Melbourne, Fla.
\MR{0698779}


\bibitem{Fogarty}
\textsc{Fogarty, C.B. and Small, D.S.} (2014). Equivalence testing for functional data with an application to comparing pulmonary function devices. \textit{The Annals of Applied Statistics}
\textbf{8}(4) 2002--2026.
\MR{3292487}


%\bibitem{Friz/Hairer}
%\textsc{Friz, P. and Hairer, M.} (2014). \textit{A course on rough paths}, Universitext
%Springer, Cham.
%\MR{3289027}


%\bibitem{Friz/Victoir}
%\textsc{Friz, P. and Victoir, N.} (2010). \textit{Multidimensional stochastic processes as rough paths}, Cambridge Studies in Advanced Mathematics, 120
%Cambridge University Press, Cambridge.
%\MR{2604669}


%\bibitem{Gatheral}
%\textsc{Gatheral, J., Jaisson, T. and Rosenbaum, M.} (2018). 
%Volatility is rough. \textit{Quantitative Finance}
%\textbf{18}(6) 933–-949.
%\MR{3805308}


%\bibitem{Gobet}
%\textsc{Gobet, E., Hoffmann, M. and Reiß, M.} (2004). 
%Nonparametric estimation of scalar diffusions based on low frequency data. %\textit{The Annals of Statistics 32(5)}
%\textbf{3} 2223–-2253.
%\MR{2102509}


\bibitem{Ingster1}
\textsc{Ingster, Y.I.} (1982). 
Minimax nonparametric detection of signals in white Gaussian noise. \textit{Problems Inform. Transmission}
\textbf{18} 130–-140.
\MR{0689340}


\bibitem{Ingster2}
\textsc{Ingster, Y.I.} (1993). 
Asymptotically minimax hypothesis testing for nonparametric alternatives I-III. \textit{Mathematical Methods of Statistics}
\textbf{2} 85–-114, 171--189, 249--268.
\MR{1257978} \MR{1257983} \MR{1259685}


\bibitem{Kallenberg}
\textsc{Kallenberg, O.} (2021). \textit{Foundations of modern probability}, 3rd ed. Probability Theory and Stochastic Modelling, 99.
Springer, Cham.
\MR{4226142}


\bibitem{Karatzas/Shreve}
\textsc{Karatzas, I. and Shreve, S.E.} (2000). \textit{Brownian motion and stochastic calculus}, 2nd ed. Graduate Texts in Mathematics 113
Springer, New York.
\MR{1121940}


\bibitem{Kasy}
\textsc{Kasy, M.} (2019).
Uniformity and the delta method. \textit{Journal of Econometric Methods}
\textbf{8}(1) 19 pp.
\MR{3898233}


\bibitem{Klenke}
\textsc{Klenke, A.} (2020). \textit{Probability Theory - A Comprehensive Course}, 3rd ed. Universitext. Springer, Cham
\MR{4201399}


\bibitem{Kloeden}
\textsc{Kloeden, P.E. and Platen, E.} (1992). \textit{Numerical solution of stochastic differential equations}, Applications of Mathematics (New York), 23. Springer, Berlin.
\MR{1214374}


\bibitem{KKT}
\textsc{Komlós, J., Major, P. and Tusnády, G.} (1975). 
An approximation of partial sums of independent RV's and the sample DF. I. \textit{Zeitung für Wahrscheinlichkeitstheorie und Verwandte Gebiete}
\textbf{32} 111--131
\MR{0375412}


\bibitem{Koenig}
\textsc{K\"{o}nig, C., Munk, A. and Werner, F.} (2020). 
Multidimensional multiscale scanning in exponential families: limit theory and statistical consequences. \textit{The Annals of Statistics}
\textbf{48}(2) 655--678
\MR{4102671}


\bibitem{Kutoyants}
\textsc{Kutoyants, Y.A.} (2004). \textit{Statistical inference for ergodic diffusion processes},  Springer Series in Statistics,
Springer, New York.
\MR{2144185}


%\bibitem{Kutoyants2}
%\textsc{Kutoyants, Y.A.} (1984). \textit{Parameter estimation for stochastic processes},  Research and expositions in mathematics 6,
%Heldermann Verlag, Berlin. Translated from the Russian and edited by B. L. S. Prakasa Rao
%\MR{0777685}


\bibitem{Leadbetter}
\textsc{Leadbetter, M.R. and Lindgren, G. and Rootz\`{e}n, H.} (1983). \textit{Extremes and related properties of random sequences and processes},  Springer Series in Statistics,
Springer, New York-Berlin.
\MR{0691492}


%\bibitem{Talagrand}
%\textsc{Ledoux, M. and Talagrand, M.} (1991). \textit{Probability in Banach spaces. Isoperimetry and processes},  Ergebnisse der Mathematik und ihrer Grenzgebiete (3), Band 23.
%Springer, Berlin.
%\MR{1102015}



\bibitem{Leonov}
\textsc{Leonov, S.L.} (1999).
Remarks on extremal problems in nonparametric curve estimation. \textit{Statistics and Probability Letters}
\textbf{43} 169--178.
\MR{1693289}


%\bibitem{Lepski/Tsybakov}
%\textsc{Lepski, S.L. and Tsybakov, A.}(2000).
%Asymptotically exact nonparametric hypothesis testing in sup-norm and at a fixed point.
%\textit{Probability Theory and Related Fields}
%\textbf{117} 17-48
%\MR{1759508}


%\bibitem{Lyons}
%\textsc{Lyons, T.} (1998).
%Differential equations driven by rough signals. \textit{Rev. Mat. Iberoamericana}
%\textbf{14}(2) 215--310.
%\MR{1654527}


%\bibitem{Mishura}
%\textsc{Mishura, Y.} (2008). \textit{Stochastic calculus for fractional Brownian motion and related processes.}, Lecture Notes in Mathematics 1929
%Springer, Berlin.
%\MR{2378138}


\bibitem{McBride}
\textsc{McBride, G.B.} (1999).
Equivalence tests can enhance environmental science and management. \textit{Australian \& New Zealand Journal of Statistics}
\textbf{41}(1) 19--29.
%\MR{???}


\bibitem{Mendy}
\textsc{Mendy, S.T.} (2009). \textit{Quasi-stationarity of stochastic models for the spread of infectious diseases}, PhD thesis, University of Liverpool.


\bibitem{Nikiforov}
\textsc{Nikiforov, A.F. and Uvarov, V.B.} (1988). \textit{Special functions of mathematical physics. A unified introduction with applications}, translated from the Russian and with a preface by Ralph P. Boas. With a foreword by A. A. Samarskiĭ,
Birhäuser Verlag, Basel
\MR{0922041}


\bibitem{Nualart}
\textsc{Nualart, D. and Ouknine, Y.} (2002).
Regularization of differential equations by fractional noise. \textit{Stochastic Processes and their Applications}
\textbf{102} 103--116.
\MR{1934157}


\bibitem{Proksch}
\textsc{Proksch, K., Munk, A. and Werner, F.} (2018).
Multiscale scanning in inverse problems. \textit{The Annals of Statistics}
\textbf{46}(6B) 3569--3602.
\MR{3852662}


\bibitem{Rohde_Diss}
\textsc{Rohde, A.} (2006).
New multiscale approaches to nonparametric statistical inference. \textit{Dissertation, Universität Bern}
\textbf{3} 515--559.
%\MR{}


\bibitem{Rohde_2}
\textsc{Rohde, A.} (2008).
Adaptive goodness-of-fit test based on signed ranks. \textit{The Annals of Statistics}
\textbf{36}(3) 1346--1374.
\MR{2418660}


\bibitem{Rohde}
\textsc{Rohde, A.} (2011).
Optimal calibration for multiple testing against local inhomogeneity in higher dimension. \textit{Probability Theory and Related Fields}
\textbf{149}(3-4) 515--559.
\MR{2776625}


\bibitem{Romano}
\textsc{Romano, J.P.} (2005).
Optimal testing of equivalence hypotheses. \textit{The Annals of Statistics}
\textbf{33}(3) 1036--1047.
\MR{2195627}


\bibitem{Rudin}
\textsc{Rudin, W.} (1964). \textit{Principles of mathematical analysis.}, 2nd ed.
McGraw-Hill Book Co. New York
\MR{0166310}


\bibitem{Samko}
\textsc{Samko, S.G., Kilbas, A.A. and Marichev, O.I.} (1993). \textit{Fractional Integrals and Derivatives},
Gordon and Breach Science
\MR{1347689}


\bibitem{Saussereau}
\textsc{Saussereau, B.} (2012).
Transportation inequalities for stochastic differential equations driven by a fractional Brownian motion. \textit{Bernoulli}
\textbf{18}(1) 1--23.
\MR{2888696}


\bibitem{Spokoiny}
\textsc{Spokoiny, V.G.} (2000).
Adaptive drift estimation for nonparametric diffusion model. \textit{The Annals of Statistics}
\textbf{28} 815--836.
\MR{1792788}


\bibitem{Strauch_2}
\textsc{Strauch, C.} (2016).
Exact adaptive pointwise drift estimation for multidimensional ergodic diffusions. \textit{Probability Theory and Related Fields}
\textbf{164}(1-2) 361--400.
\MR{3449393}


\bibitem{Strauch_3}
\textsc{Strauch, C.} (2018).
Adaptive invariant density estimation for ergodic diffusions over anisotropic classes. \textit{The Annals of Statistics}
\textbf{48}(6B) 3451--3480.
\MR{3852658}


\bibitem{Tudor}
\textsc{Tudor, C.A. and Viens, F.G.} (2007).
Statistical aspects of the fractional stochastic calculus. \textit{The Annals of Statistics}
\textbf{35}(3) 1183--1212.
\MR{2341703}


%\bibitem{vanZanten}
%\textsc{van Zanten, H.} (2003).
%On Uniform Laws of large numbers for ergodic diffusions and consistency of estimators. \textit{Statistical Inference for Stochastic Processes}
%\textbf{6} 199--213.
%\MR{1984775}


%\bibitem{vanZanten_2}
%\textsc{van Zanten, H.} (2000).
%On uniform convergence of the empirical density of an ergodic diffusion. \textit{Statistical Inference for Stochastic Processes}
%\textbf{3} 251--262.
%\MR{1819398}


\bibitem{Wellek}
\textsc{Wellek, S.} (2010). \textit{Testing statistical hypotheses of equivalence and noninferiority}, 2nd ed.
CRC Press, Boca Raton
\MR{267002}


\bibitem{Wellner}
\textsc{van der Vaart, A.W. and Wellner, J.A.} (1996). \textit{Weak convergence and empirical processes},  Springer Series in Statistics,
Springer, New York.
\MR{1385671}


\end{thebibliography}








\newpage
\setcounter{section}{0}
\renewcommand*\thesection{\Alph{section}}



\input{Sections/Intro_App}
\input{Sections/Appendix_Implementation}
\input{Sections/Appendix_Example_SIS}
\input{Sections/Appendix_Preliminary_lemma}
\input{Sections/Appendix_multiscale}
\input{Sections/Appendix_Weak_conv}
\input{Sections/Appendix_least}
\input{Sections/Appendix_lower}
%\input{Sections/Appendix_upper}
%\include{Sections/Appendix_composite}
\input{Sections/Appendix_stability}
%\include{Sections/TrialsII}




\vspace{2cm}
\small{
\hspace{-0.4cm}\textsc{Institute of Mathematics}\\
\textsc{University of Freiburg}\\
\textsc{Ernst-Zermelo-Strasse 1}\\
\textsc{79104 Freiburg}\\
\textsc{Germany}\\
\textsc{E-Mail:} johannes.brutsche@stochastik.uni-freiburg.de\\
\textcolor{white}{\textsc{E-Mail:}} angelika.rohde@stochastik.uni-freiburg.de}




\end{document}
