# Supplementary material for: Sharp adaptive and pathwise stable similarity testing for scalar ergodic diffusions
Source: arXiv:2203.13776 source file (2024-04-16)
Supplement: Supplementary file 13 [file Appendix_Example_SIS.tex]

\section{The context of diffusions as scaling limits, tolerant testing in the diffusion model and the stability of the test}\label{App_SIS}


%The following example is well-known but may provide an insightful supplement to our presentation.
The aim of this section is to illustrate on the basis of the stochastic SIS model the interplay of similarity testing in the diffusion approximation and the stability property.

\subsection{The stochastic SIS model and its diffusion scaling limit}\label{SubSec_SIS}
We consider a population of size $N$ consisting of susceptible~(S) and infected (I) people. The SIS model is characterized by two possible events, namely that a susceptible individuum gets infected when meeting an infected individuum and an infected one recovers and is again susceptible. This is described via a contact rate $\alpha$ and a recovery rate $\beta$, see Chapter~$3$ in~\cite{Mendy}. %The SIS model can then be characterized via the reactions
%\[ S + I \stackrel{\alpha}{\longrightarrow} 2I, \qquad I\stackrel{\beta}{\longrightarrow} S\]
%meaning that at reaction rate constant $\alpha$ an infected and one susceptible person are turned into two infected peole and at reaction rate $\beta$, an infected person recovers and is again susceptible. Denoting $I^N=(I^N(t))_{t\geq 0}$ and using two unit-rate Poisson processes $Y_1$ and $Y_2$, the above reactions lead to the time-change equation
Denote $I_{\alpha,\beta}^N  =(I_{\alpha,\beta}^N(t))_{t\geq 0}$ the number of infected people in a population of size $N$. Then this number is given in the SIS model by the time-change equation {\small 
\[ I_{\alpha,\beta}^N(t) = I_{\alpha,\beta}^N(0) + Y_1\left( \alpha \int_0^t I_{\alpha,\beta}^N(s) (1-I_{\alpha,\beta}^N(s)/N)ds\right) - Y_2\left( \beta\int_0^t I_{\alpha,\beta}^N(s)ds\right) \]}

\noindent
where $Y_1$ and $Y_2$ are two independent unit-rate Poisson processes (see Example~$2.1$ and p.21 in \cite{Anderson/Kurtz}). Let $x_{\alpha,\beta}^N:=I_{\alpha,\beta}^N/N$ be the proportion of infected people. Assuming that $I_{\alpha,\beta}^N(0)/N \rightarrow x_{\alpha,\beta}(0)$ as $N\to\infty$ for some $x_{\alpha,\beta}(0)\in\R$, Theorem~$4.1$ in \cite{Anderson/Kurtz} shows that $(x_{\alpha,\beta}^N)_{N\in\N}$ converges uniformly on compact sets in probability to the solution $x_{\alpha,\beta}$ of
\[  x_{\alpha,\beta}(t) = x_{\alpha,\beta}(0) + \int_0^t \alpha x_{\alpha,\beta}(s)(1-x_{\alpha,\beta}(s)) - \beta x_{\alpha,\beta}(s) ds.\]
This evolution equation has $x_{\alpha,\beta}^* =0$ and $x_{\alpha,\beta}^*=\frac{\alpha-\beta}{\alpha}$ as equilibria. Moreover, the process 
\[ U_{\alpha,\beta}^N := \sqrt{N}(x_{\alpha,\beta}^N-x_{\alpha,\beta}) \] 
converges weakly to $U_{\alpha,\beta}=(U_{\alpha,\beta}(t))_{t\geq 0}$ solving {\small
\begin{align*}
 U_{\alpha,\beta}(t) &= U_{\alpha,\beta}(0) + W_1\left(\alpha\int_0^t x_{\alpha,\beta}(s)(1-x_{\alpha,\beta}(s))ds\right)
+W_2\left( \beta \int_0^t x_{\alpha,\beta}(s) ds\right)\\
&\hspace{3cm} + \int_0^t \alpha (1-2x_{\alpha,\beta}(s))U_{\alpha,\beta}(s) - \beta U_{\alpha,\beta}(s)ds
\end{align*}}

\noindent
with two independent Brownian motions $W_1$ and $W_2$ (see $(4.8)$ and its derivation in \cite{Anderson/Kurtz}).
%Moreover, since
%\[ \left( \sqrt{N}\left(\frac1N Y_i(Nt) - t\right)\right)_{t\geq 0}\stackrel{N\to\infty}{\longrightarrow}_{\mathcal{D}} W\]
%for a Brownian motion $W$, we find that $U^N:=\sqrt{N}(x^N-x)$ with
%\begin{align*}
%U^N(t) &= U^N(0) + \sqrt{N}\left( \frac1N Y_1\left( \alpha N\int_0^t x^N(s)(1-x^N(s)) ds \right)\right.\\
%&\hspace{4cm} \left.- \int_0^t \alpha x(s)(1-x(s))ds\right) \\
%&\hspace{2cm} - \sqrt{N}\left(\frac1N Y_2\left( \beta N\int_0^t x^N(s)ds\right) - \int_0^t \beta x(s)ds\right)
%\end{align*}
If $x_{\alpha,\beta}(0)= x_{\alpha,\beta}^*=\frac{\alpha-\beta}{\alpha}$, then $U_{\alpha,\beta}$ solves 
\[ dU_{\alpha,\beta}(t) = -(\alpha-\beta)U_{\alpha,\beta}(t) dt + \sqrt{\frac{2\beta(\alpha-\beta)}{\alpha}} dW(t)\] 
for some Brownian motion $W$, see also Section~$3.5$ in~\cite{Mendy} for the derivation of this Ornstein--Uhlenbeck process.
%. In other words, we have
%\[ I^N(t) = \frac{N(\alpha-\beta)}{\alpha} + \sqrt{N}U(t),\]
%where $U$ is the above Ornstein--Uhlenbeck process, 



\begin{figure}[h]
\begin{center}
\begin{tikzpicture}[>=stealth, thick] 

\node (A) at (0,0) [draw, process, text width=4cm, minimum height=0.5cm, align=flush center] 
{SIS model $U_{\alpha,\beta}^N$};

\node (B) at (0,-3) [draw, process, text width=4cm, minimum height=0.5cm, align=flush center] 
{Diffusion approximation $U_{\alpha,\beta}$};

\node (C) at (7,-3) [draw, process, text width=4cm, minimum height=0.5cm, align=flush center] 
{Nonparametric diffusion approximation $U$};

\node (D) at (7,0) [draw, process, text width=4cm, minimum height=0.5cm, align=flush center] 
{Data generating process $U^N$};

%\coordinate (z) at (0,-3);

\draw[->] (A) -- node[left] {scaling limit}(B);
\draw[<->] (B) -- node[above] {tolerance $\eta$} (C);
\draw[->] (D) -- node[right] {imposed scaling limit}(C);
\draw[dotted] (A) -- (D);
%\draw[->] (B) -- (z) -| node[above] {YES} (D);

\end{tikzpicture}\caption{Prototypical example motivating the interplay of tolerant testing in a diffusion approximation and the stability of a tolerant test.}\label{fig:tolerance_stability}
\end{center}
\end{figure}


\subsection{Tolerant testing in the diffusion approximation and stability}
Although widely used in epidemiology, the SIS model is by far too simplified in order to capture the full dynamics and can adequately describe the data at most within a certain tolerance. Suppose we want to infer on deviations of the SIS model $U_{\alpha,\beta}^N$ from the real phenomenon $U^N$ within tolerance $\eta$. Imposing that $U^N$ likewise has a diffusion approximation $U$ motivates applying a similarity test developed for diffusion models, i.e. to test the tolerant null hypothesis against the alternative that $U_{\alpha,\beta}$ deviates from $U$ at tolerance $\eta$, see Figure~\ref{fig:tolerance_stability}. This approach is indeed justified by a stability property with respect to the diffusion approximation which allows to transfer (at least for large $N$ and within some small error) the results of the test for the diffusion model to the original jump process model. Note that in this example, such stability has to cover approximation schemes with laws singular to the one of the diffusion limit as the law $\mathcal{L}(U_{\alpha,\beta}^N)$ of $U_{\alpha,\beta}^N$ is singular to the law $\mathcal{L}(U_{\alpha,\beta})$ of $U_{\alpha,\beta}$ - even after linear interpolation to make the sample paths continuous. 
